# Supplementary material for: Dynamic Chemical Model for H2/O2 Combustion Developed Through a Community Workflow
Source: arXiv:1801.10093 ancillary file (2018-02-03)
Supplement: Supplementary file 1 [file supplementaryMaterial.pdf]

# Supplementary Material
# Dynamic Chemical Model for $H_2/O_2$ Combustion Developed Through a Community Workflow

James Oreluk[a], Craig D. Needham[b], Sathya Baskaran[c], S. Mani Sarathy[c], Michael P. Burke[d], Richard H. West[e], Michael Frenklach[a], Phillip R. Westmoreland[b]

[a]*Department of Mechanical Engineering, University of California, Berkeley, CA 94720, USA*
[b]*Department of Chemical & Biomolecular Engineering, North Carolina State University, Raleigh, NC 27695-7905, USA*
[c]*King Abdullah University of Science and Technology, Thuwal, Saudi Arabia*
[d]*Department of Mechanical Engineering, Department of Chemical Engineering, and Data Science Institute, Columbia University, New York, NY 10027, USA*
[e]*Department of Chemical Engineering, Northeastern University, Boston, MA 02115, USA*

---

---

### QOIs used in the study

**Table S1.** Experimental shock-tube ignition-delay QOIs.
**Table S2.** Experimental flame-speed QOIs.
**Figure S1.** Screenshot of HDF5 input file of species.
**Figure S2.** Screenshot of HDF5 input file of reactions.
**Figure S3.** Screenshot of HDF5 input file of Arrhenius parameters.

### Ignition-delay Simulations

**Table S3.** Comparison of ignition-delay results for Mechanism1, Mechanism2, Mechanism3, and DynamicMech151203.
**Table S4.** $\ell_2$-norm of the difference between each mechanisms prediction, $M(x)$, to the measured ignition delay, $\tau_{\text{ign}}$.

### Flame Simulations

**Figure S4.** Screenshot of HDF5 simulation output for calculated flame speed.

**Figure S5.** Screenshot of HDF5 simulation output for distance, velocity, and density details.
**Figure S6.** Screenshot of HDF5 simulation output for species concentrations.
**Table S5.** Comparison of flame-speed results (multicomponent transport with Soret effect) for Mechanism1, Mechanism2, Mechanism3, and DynamicMech151203.
**Table S6.** Comparison of flame-speed results (mixture-averaged transport) with CloudFlame-Cantera and CHEMKIN-PRO for Mechanism1.

### Consistency Analysis

**Figure S7.** Normalized sensitivity of the consistency measure with respect to parameter bounds. Blue bars indicate sensitivity to a parameters lower bound ($L_e$), and red bars are upper bounds ($U_e$), where $e$ is the parameter index. Sensitivities of the consistency measure to the experimental bounds shown in Figure 2 in the paper are an order of magnitude larger than those of the parameter bounds. Therefore, we examined the experimental bounds to resolve the inconsistency.

### Cantera Input Files

**Mechanism1 -** `m00000007.cti`
**Mechanism2 -** `m00000008.cti`
**Mechanism3 -** `m00000009.cti`
**DynamicMech151203 -** `m00000010.cti`

---

## 1. QOIs used in the study

Table S1: Experimental shock-tube ignition-delay QOIs.

| Equiv ratio $\Phi$ | P [atm] | T [K] | $\tau_{ign}$ [ms] | Uncertainty Bounds of $\tau_{ign}$ | | PrIMe ID | Ref |
|---|---|---|---|---|---|---|---|
| 0.17 | 0.32 | 2007 | 0.0426 | 0.0201 | 0.0903 | a00000451* | [1] |
| | | 1768 | 0.0756 | 0.0365 | 0.1565 | a00000452* | |
| | | 1580 | 0.1341 | 0.0637 | 0.2825 | a00000453* | |
| 0.50 | 0.34 | 2224 | 0.0662 | 0.0460 | 0.0951 | a00000448* | [1] |
| | | 1969 | 0.1063 | 0.0750 | 0.1507 | a00000449* | |
| | | 1767 | 0.1709 | 0.1184 | 0.2466 | a00000450* | |
| 1.50 | 0.33 | 2090 | 0.0461 | 0.0276 | 0.0768 | a00000445* | [1] |
| | | 1838 | 0.0829 | 0.0511 | 0.1346 | a00000446* | |
| | | 1640 | 0.1493 | 0.0912 | 0.2444 | a00000447* | |
| 0.39 | 2.18 | 1412 | 0.1392 | 0.0840 | 0.2306 | a00000382* | [2] |
| | | 1318 | 0.2096 | 0.1280 | 0.3433 | a00000383* | |
| | | 1237 | 0.3157 | 0.1916 | 0.5201 | a00000384* | |
| 0.75 | 2.10 | 1311 | 0.2494 | 0.1131 | 0.5500 | a00000385 | [2] |
| | | 1266 | 0.3113 | 0.1423 | 0.6808 | a00000386* | |
| | | 1223 | 0.3885 | 0.1740 | 0.8676 | a00000387* | |
| 1.00 | 2.04 | 1299 | 0.3125 | 0.1338 | 0.7296 | a00000454* | [2] |
| | | 1257 | 0.3659 | 0.1626 | 0.8234 | a00000455* | |
| | | 1218 | 0.4284 | 0.1916 | 0.9579 | a00000456* | |
| 1.00 | 1.94 | 1454 | 0.0273 | 0.0192 | 0.0390 | a00000370* | [3] |
| | | 1269 | 0.0616 | 0.0438 | 0.0866 | a00000371* | |
| | | 1126 | 0.1386 | 0.0988 | 0.1946 | a00000372* | |
| 1.00 | 0.71 | 1352 | 0.0498 | 0.0308 | 0.0806 | a00000373 | [4] |
| | | 1180 | 0.0992 | 0.0621 | 0.1585 | a00000374 | |
| | | 1047 | 0.1977 | 0.1234 | 0.3168 | a00000375 | |
| 1.00 | 1.45 | 1161 | 0.2021 | 0.0880 | 0.4637 | a00000460* | [5] |
| | | 1027 | 0.4783 | 0.2087 | 1.0961 | a00000461* | |
| | | 921 | 1.1324 | 0.4753 | 2.6977 | a00000462* | |
| 1.00 | 2.35 | 1023 | 0.2167 | 0.0997 | 0.4711 | a00000463* | [5] |
| | | 974 | 0.4857 | 0.2323 | 1.0156 | a00000464 | |
| | | 930 | 1.0888 | 0.5212 | 2.2747 | a00000465 | |
| 0.50 | 1.05 | 999 | 1.0014 | 0.7424 | 1.3508 | a00000388 | [6] |
| | | 972 | 1.4996 | 1.1135 | 2.0195 | a00000389 | |

Table S1: Experimental shock-tube ignition-delay QOIs.

| Equiv ratio Φ | P [atm] | T [K] | $\tau_{ign}$ [ms] | Uncertainty Bounds of $\tau_{ign}$ | | PrIMe ID | Ref |
|---|---|---|---|---|---|---|---|
| | | 947 | 2.2456 | 1.6521 | 3.0525 | a00000390 | |
| | | 1015 | 0.7533 | 0.4799 | 1.1826 | a00000391 | |
| 0.50 | 3.99 | 995 | 1.4457 | 0.9244 | 2.2609 | a00000392* | [6] |
| | | 976 | 2.7743 | 1.7571 | 4.3804 | a00000393* | |
| | | 1093 | 0.8912 | 0.7036 | 1.1288 | a00000394 | |
| 0.50 | 15.86 | 1067 | 1.5758 | 1.2490 | 1.9882 | a00000395 | [6] |
| | | 1042 | 2.7864 | 2.1811 | 3.5596 | a00000396 | |
| | | 1411 | 0.1112 | 0.0760 | 0.1628 | a00000415* | |
| 1.00 | 1.01 | 1197 | 0.2988 | 0.2062 | 0.4329 | a00000416 | [6] |
| | | 1039 | 0.8025 | 0.5445 | 1.1829 | a00000417 | |
| | | 1103 | 0.1333 | 0.0563 | 0.3153 | a00000418 | |
| 1.00 | 3.96 | 1052 | 0.3919 | 0.1708 | 0.8992 | a00000419 | [6] |
| | | 1005 | 1.1528 | 0.4936 | 2.6926 | a00000420 | |
| | | 1174 | 0.0505 | 0.0359 | 0.0711 | a00000421 | |
| 1.00 | 16.39 | 1115 | 0.2506 | 0.1786 | 0.3517 | a00000422 | [6] |
| | | 1063 | 1.2436 | 0.8793 | 1.7590 | a00000423* | |
| | | 1221 | 0.0739 | 0.0204 | 0.2675 | a00000439* | |
| 0.10 | 3.69 | 1108 | 0.3037 | 0.0866 | 1.0650 | a00000440 | [7] |
| | | 1014 | 1.2486 | 0.3554 | 4.3863 | a00000441* | |
| | | 1372 | 0.0410 | 0.0300 | 0.0560 | a00000427 | |
| 0.10 | 1.01 | 1162 | 0.1455 | 0.1085 | 0.1950 | a00000428 | [7] |
| | | 1007 | 0.5158 | 0.3859 | 0.6894 | a00000429 | |
| | | 1074 | 0.1147 | 0.0471 | 0.2792 | a00000430 | |
| 0.10 | 4.17 | 1022 | 0.4968 | 0.2112 | 1.1687 | a00000431* | [7] |
| | | 975 | 2.1530 | 0.9012 | 5.1438 | a00000432* | |
| | | 1113 | 0.3755 | 0.1473 | 0.9572 | a00000433* | |
| 0.10 | 17.78 | 1055 | 1.0493 | 0.4138 | 2.6609 | a00000434 | [7] |
| | | 1003 | 2.9324 | 1.1114 | 7.7368 | a00000435 | |
| | | 1608 | 0.0810 | 0.0279 | 0.2350 | a00000436 | |
| 0.10 | 0.94 | 1299 | 0.2626 | 0.0930 | 0.7416 | a00000437* | [7] |
| | | 1090 | 0.8520 | 0.3000 | 2.4195 | a00000438 | |
| | | 1192 | 0.1241 | 0.0579 | 0.2660 | a00000442 | |
| 0.10 | 16.31 | 1136 | 0.5109 | 0.2456 | 1.0629 | a00000443* | [7] |
| | | 1084 | 2.1028 | 1.0091 | 4.3820 | a00000444* | |

Table S1: Experimental shock-tube ignition-delay QOIs.

| Equiv ratio Φ | P [atm] | T [K] | $\tau_{ign}$ [ms] | Uncertainty Bounds of $\tau_{ign}$ | | PrIMe ID | Ref |
|---|---|---|---|---|---|---|---|
| | | 1534 | 0.0811 | 0.0509 | 0.1292 | a00000397 | |
| 0.50 | 0.99 | 1262 | 0.2668 | 0.1709 | 0.4167 | a00000398 | [7] |
| | | 1072 | 0.8779 | 0.5654 | 1.3630 | a00000399 | |
| | | 1183 | 0.0939 | 0.0417 | 0.2116 | a00000400 | |
| 0.50 | 4.08 | 1118 | 0.3172 | 0.1446 | 0.6960 | a00000401* | [7] |
| | | 1059 | 1.0718 | 0.4861 | 2.3631 | a00000402* | |
| | | 1192 | 0.1853 | 0.1101 | 0.3117 | a00000403 | |
| 0.50 | 15.57 | 1144 | 0.5729 | 0.3427 | 0.9576 | a00000404 | [7] |
| | | 1101 | 1.7710 | 1.0402 | 3.0153 | a00000405 | |
| | | 1623 | 0.0849 | 0.0280 | 0.2577 | a00000406* | |
| 3.99 | 1.06 | 1308 | 0.2522 | 0.0883 | 0.7208 | a00000407 | [7] |
| | | 1096 | 0.7491 | 0.2651 | 2.1165 | a00000408 | |
| | | 1297 | 0.0565 | 0.0136 | 0.2351 | a00000409 | |
| 3.99 | 3.98 | 1164 | 0.1954 | 0.0483 | 0.7897 | a00000410 | [7] |
| | | 1057 | 0.6756 | 0.1623 | 2.8127 | a00000411* | |
| | | 1143 | 0.1697 | 0.0979 | 0.2941 | a00000412 | |
| 3.99 | 14.87 | 1069 | 0.7237 | 0.4231 | 1.2381 | a00000413 | [7] |
| | | 1004 | 3.0870 | 1.7975 | 5.3016 | a00000414 | |
| | | 1009 | 0.2344 | 0.1048 | 0.5244 | a00000457 | |
| 0.42 | 3.28 | 972 | 0.8252 | 0.3762 | 1.8102 | a00000458* | [8] |
| | | 938 | 2.9051 | 1.2947 | 6.5184 | a00000459* | |
| | | 1062 | 0.3217 | 0.1535 | 0.6742 | a00000376 | |
| 1.00 | 3.56 | 1012 | 1.0194 | 0.4931 | 2.1072 | a00000377* | [8] |
| | | 966 | 3.2307 | 1.5479 | 6.7428 | a00000378* | |
| | | 1296 | 0.2278 | 0.1284 | 0.4041 | a00000466 | |
| 1.00 | 1.00 | 1184 | 0.3902 | 0.2287 | 0.6657 | a00000467 | [9] |
| | | 1089 | 0.6685 | 0.3927 | 1.1379 | a00000468 | |
| | | 1564 | 0.1707 | 0.1630 | 0.1787 | a00000472 | |
| 1.03 | 1.00 | 1411 | 0.3018 | 0.2893 | 0.3149 | a00000473 | [9] |
| | | 1286 | 0.5337 | 0.5118 | 0.5566 | a00000474* | |
| | | 1386 | 0.1634 | 0.1407 | 0.1898 | a00000469* | |
| 1.47 | 1.00 | 1280 | 0.2403 | 0.2089 | 0.2763 | a00000470* | [9] |
| | | 1190 | 0.3532 | 0.3071 | 0.4062 | a00000471* | |
| | | 1270 | 0.0263 | 0.0230 | 0.0300 | a00000361 | |

Table S1: Experimental shock-tube ignition-delay QOIs.

| **Equiv ratio Φ** | **P [atm]** | **T [K]** | $\tau_{\mathrm{ign}}$ **[ms]** | **Uncertainty Bounds of** $\tau_{\mathrm{ign}}$ | | **PrIMe ID** | **Ref** |
|---|---|---|---|---|---|---|---|
| 1.00 | 33.00 | 1242 | 0.0592 | 0.0519 | 0.0676 | a00000362 | [10] |
| | | 1215 | 0.1337 | 0.1168 | 0.1529 | a00000363 | |
| | | 1714 | 0.0235 | 0.0176 | 0.0315 | a00000364 | |
| 1.00 | 64.00 | 1578 | 0.0423 | 0.0320 | 0.0558 | a00000365 | [10] |
| | | 1461 | 0.0760 | 0.0569 | 0.1013 | a00000366 | |
| | | 1327 | 0.1031 | 0.0866 | 0.1226 | a00000367 | |
| 1.00 | 64.00 | 1311 | 0.1438 | 0.1220 | 0.1695 | a00000368* | [10] |
| | | 1295 | 0.2007 | 0.1695 | 0.2376 | a00000369* | |
| | | 1566 | 0.0668 | 0.0283 | 0.1576 | a00000424 | |
| 0.25 | 1.32 | 1365 | 0.1137 | 0.0502 | 0.2575 | a00000425 | [11] |
| | | 1210 | 0.1933 | 0.0856 | 0.4366 | a00000426* | |
| | | 1045 | 0.5000 | 0.3152 | 0.7931 | a00000379 | |
| 2.00 | 5.00 | 1016 | 1.3800 | 0.8768 | 2.1720 | a00000380 | [12] |
| | | 990 | 3.8100 | 2.3867 | 6.0823 | a00000381 | |

* Indicates target was not included in final, reduced dataset.

Table S2: Experimental flame-speed QOIs.

| Φ | **Pressure [atm]** | **Flame speed [cm/s]** | **PrIMe ID** | **Ref** |
|---|---|---|---|---|
| 0.6 | 1 | 81.88 | a00000476 | |
| 0.85 | 10 | 45.3 | a00000483 | |
| 0.85 | 15 | 26.9 | a00000482 | |
| 0.85 | 20 | 18.35 | a00000481 | |
| 1.5 | 20 | 80.9 | a00000479 | [13] |
| 1.65 | 1 | 280.21 | a00000477 | |
| 2 | 20 | 64.05 | a00000480 | |
| 4 | 1 | 165.29 | a00000478 | |
| 2.5 | 15 | 28.7 | a00000484 | [14] |
| 2.5 | 25 | 27.7 | a00000485 | |

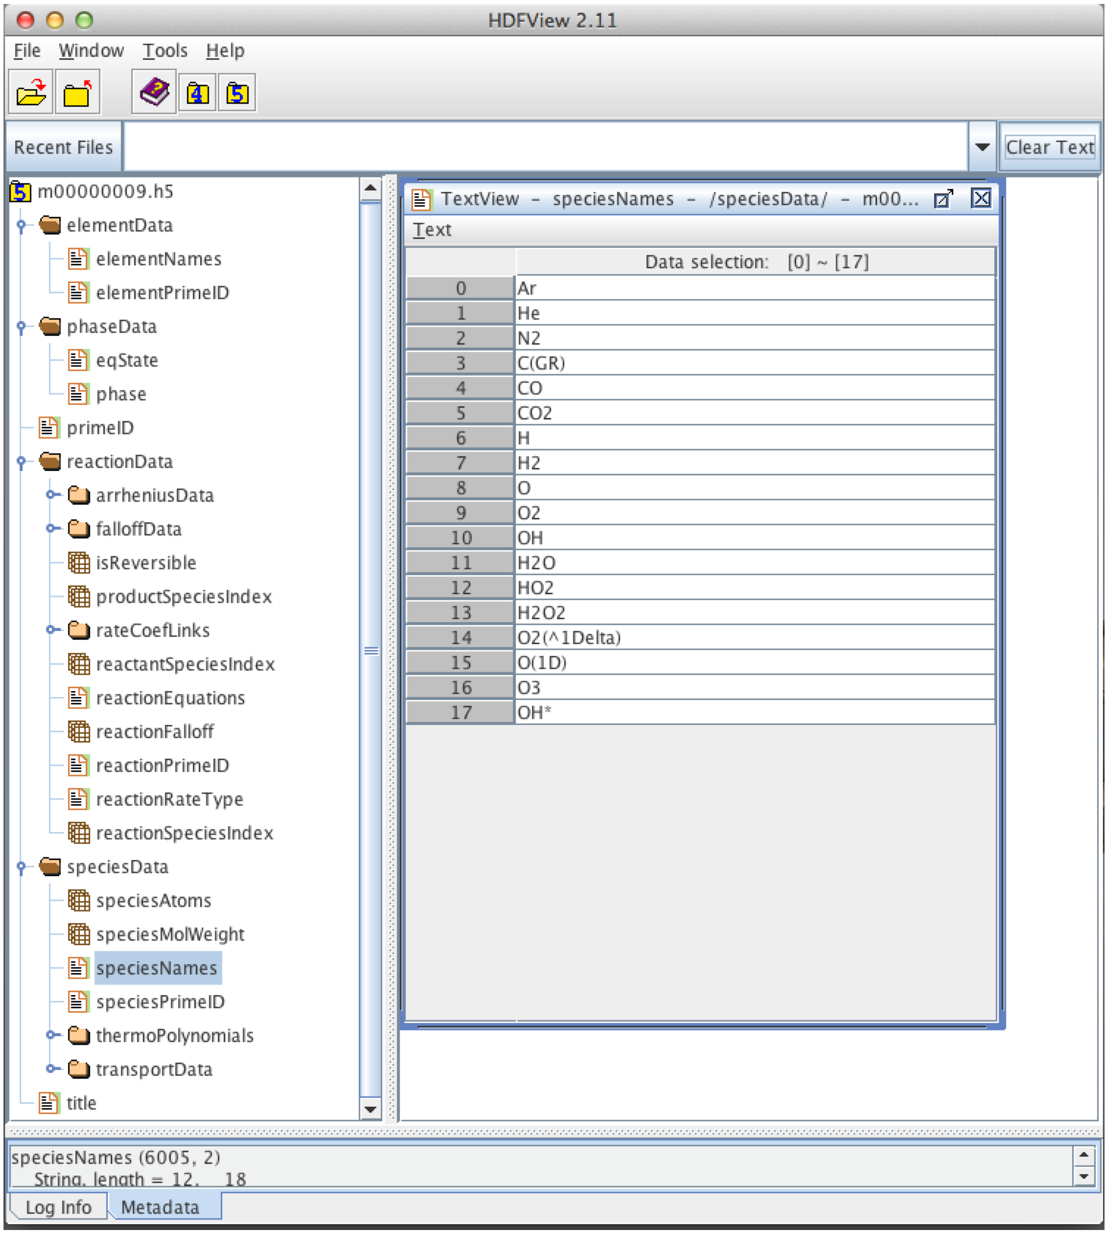


Figure S1: Screenshot of HDF5 input file of species.

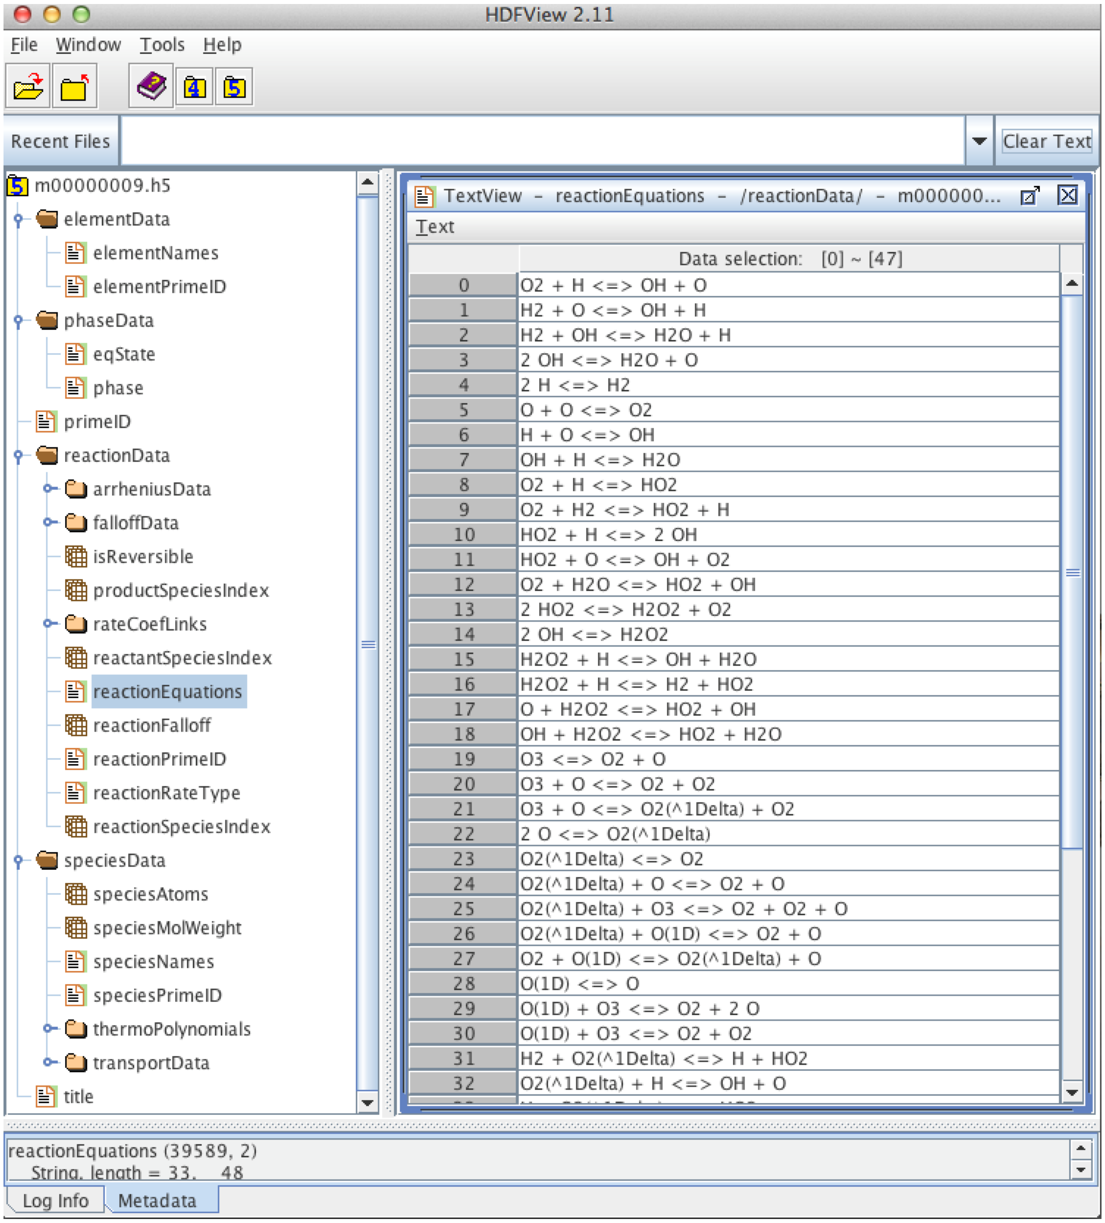


Figure S2: Screenshot of HDF5 input file of reactions.

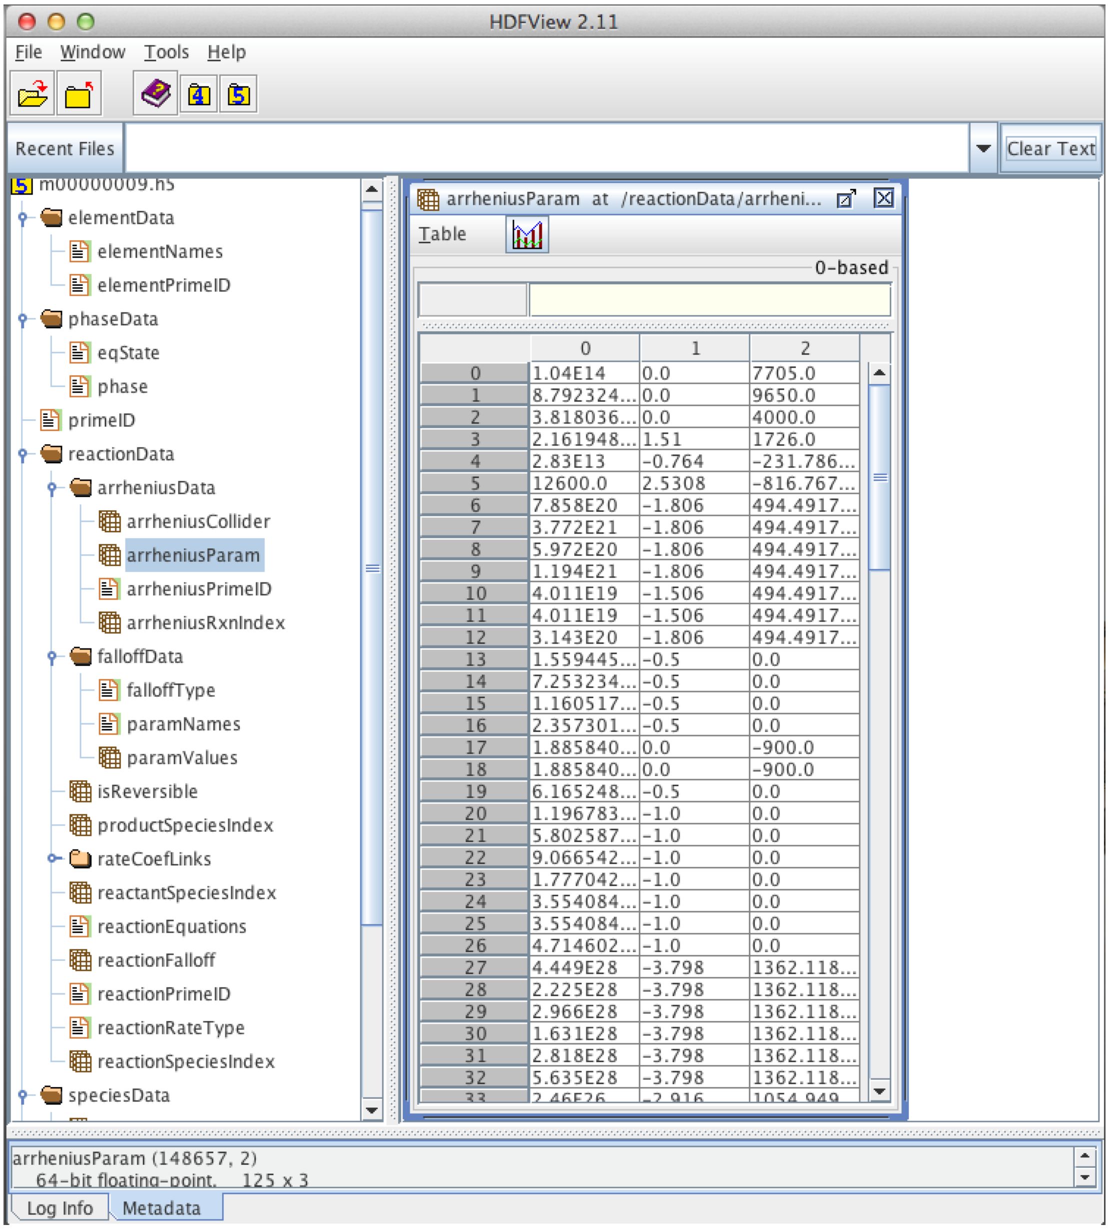

Figure S3: Screenshot of HDF5 input file of Arrhenius parameters.

## 2. Ignition-delay Simulations

Table S3: Comparison of ignition-delay results for Mechanism1, Mechanism2, Mechanism3, and DynamicMech151203.

| Equiv ratio $\Phi$ | P [atm] | T [K] | $\tau_{\mathrm{ign}}$ [ms] | Mech1 [ms] | Mech2 [ms] | Mech3 [ms] | Dynamic Mech [ms] | PrIMe ID | Ref |
|---|---|---|---|---|---|---|---|---|---|
| 0.17 | 0.32 | 2007 | 0.0426 | 0.2110 | 0.1787 | 0.2109 | 0.1668 | a00000451* | [1] |
| | | 1768 | 0.0756 | 0.2906 | 0.2437 | 0.2486 | 0.2291 | a00000452* | |
| | | 1580 | 0.1341 | 0.3530 | 0.3551 | 0.3526 | 0.3429 | a00000453* | |
| 0.50 | 0.34 | 2224 | 0.0662 | 0.1084 | 0.1086 | 0.1079 | 0.1089 | a00000448* | [1] |
| | | 1969 | 0.1063 | 0.1859 | 0.1861 | 0.1871 | 0.1923 | a00000449* | |
| | | 1767 | 0.1709 | 0.3106 | 0.3104 | 0.3084 | 0.3135 | a00000450* | |
| 1.50 | 0.33 | 2090 | 0.0461 | 0.1165 | 0.1158 | 0.1166 | 0.1201 | a00000445* | [1] |
| | | 1838 | 0.0829 | 0.2030 | 0.2032 | 0.2018 | 0.2091 | a00000446* | |
| | | 1640 | 0.1493 | 0.3469 | 0.3480 | 0.3454 | 0.3531 | a00000447* | |
| 0.39 | 2.18 | 1412 | 0.1392 | 0.3359 | 0.3327 | 0.3367 | 0.3274 | a00000382* | [2] |
| | | 1318 | 0.2096 | 0.4930 | 0.4887 | 0.4865 | 0.4750 | a00000383* | |
| | | 1237 | 0.3157 | 0.7197 | 0.7228 | 0.7179 | 0.6932 | a00000384* | |
| 0.75 | 2.10 | 1311 | 0.2494 | 0.6039 | 0.6004 | 0.6039 | 0.5884 | a00000385 | [2] |
| | | 1266 | 0.3113 | 0.7451 | 0.7488 | 0.7479 | 0.7267 | a00000386* | |
| | | 1223 | 0.3885 | 0.9293 | 0.9210 | 0.9330 | 0.9020 | a00000387* | |
| 1.00 | 2.04 | 1299 | 0.3125 | 0.7306 | 0.7347 | 0.7282 | 0.7221 | a00000454* | [2] |
| | | 1257 | 0.3659 | 0.8974 | 0.8928 | 0.8980 | 0.8801 | a00000455* | |
| | | 1218 | 0.4284 | 1.0875 | 1.0890 | 1.0930 | 1.0616 | a00000456* | |
| 1.00 | 1.94 | 1454 | 0.0273 | 0.0389 | 0.0388 | 0.0390 | 0.0387 | a00000370* | [3] |
| | | 1269 | 0.0616 | 0.0839 | 0.0839 | 0.0843 | 0.0825 | a00000371* | |

Table S3: Comparison of ignition-delay results for Mechanism1, Mechanism2, Mechanism3, and DynamicMech151203.

| **Equiv ratio Φ** | **P [atm]** | **T [K]** | $\tau_{ign}$ **[ms]** | **Mech1 [ms]** | **Mech2 [ms]** | **Mech3 [ms]** | **Dynamic Mech [ms]** | **PrIMe ID** | **Ref** |
|---|---|---|---|---|---|---|---|---|---|
| | | 1126 | 0.1386 | 0.1906 | 0.1902 | 0.1904 | 0.1815 | a00000372* | |
| | | 1352 | 0.0498 | 0.0501 | 0.0502 | 0.0502 | 0.0498 | a00000373 | |
| 1.00 | 0.71 | 1180 | 0.0992 | 0.1132 | 0.1131 | 0.1131 | 0.1116 | a00000374 | [4] |
| | | 1047 | 0.1977 | 0.2670 | 0.2668 | 0.2674 | 0.2562 | a00000375 | |
| | | 1161 | 0.2021 | 0.0634 | 0.0634 | 0.0636 | 0.0616 | a00000460* | |
| 1.00 | 1.45 | 1027 | 0.4783 | 0.1871 | 0.1867 | 0.1875 | 0.1659 | a00000461* | [5] |
| | | 921 | 1.1324 | 5.1721 | 5.1747 | 5.1740 | 2.3170 | a00000462* | |
| | | 1023 | 0.2167 | 0.1847 | 0.1841 | 0.1854 | 0.1368 | a00000463* | |
| 1.00 | 2.35 | 974 | 0.4857 | 2.4202 | 2.3691 | 2.3883 | 0.4586 | a00000464 | [5] |
| | | 930 | 1.0888 | 5.3892 | 4.8630 | 5.3778 | 5.2808 | a00000465 | |
| | | 999 | 1.0014 | 1.0716 | 1.0699 | 1.0739 | 0.9646 | a00000388 | |
| 0.50 | 1.05 | 972 | 1.4996 | 1.4500 | 1.4437 | 1.4532 | 1.2587 | a00000389 | [6] |
| | | 947 | 2.2456 | 2.0914 | 2.0814 | 2.0960 | 1.7005 | a00000390 | |
| | | 1015 | 0.7533 | 1.2968 | 1.2821 | 1.2986 | 0.4879 | a00000391 | |
| 0.50 | 3.99 | 995 | 1.4457 | 7.2147 | 7.2012 | 7.2180 | 1.0347 | a00000392* | [6] |
| | | 976 | 2.7743 | 13.2888 | 13.7560 | 13.8132 | 5.0978 | a00000393* | |
| | | 1093 | 0.8912 | 1.8995 | 1.8022 | 1.8478 | 0.7162 | a00000394 | |
| 0.50 | 15.86 | 1067 | 1.5758 | 3.8511 | 3.5931 | 3.6759 | 1.6318 | a00000395 | [6] |
| | | 1042 | 2.7864 | 7.2684 | 6.6861 | 6.8215 | 3.3953 | a00000396 | |
| | | 1411 | 0.1112 | 0.0988 | 0.0986 | 0.0984 | 0.0973 | a00000415* | |

Table S3: Comparison of ignition-delay results for Mechanism1, Mechanism2, Mechanism3, and DynamicMech151203.

| **Equiv ratio Φ** | **P [atm]** | **T [K]** | $\tau_{\text{ign}}$ **[ms]** | **Mech1 [ms]** | **Mech2 [ms]** | **Mech3 [ms]** | **Dynamic Mech [ms]** | **PrIMe ID** | **Ref** |
|---|---|---|---|---|---|---|---|---|---|
| 1.00 | 1.01 | 1197 | 0.2988 | 0.2638 | 0.2646 | 0.2637 | 0.2585 | a00000416 | [6] |
| | | 1039 | 0.8025 | 0.7395 | 0.7378 | 0.7398 | 0.7000 | a00000417 | |
| | | 1103 | 0.1333 | 0.1557 | 0.1552 | 0.1562 | 0.1361 | a00000418 | |
| 1.00 | 3.96 | 1052 | 0.3919 | 0.3219 | 0.3207 | 0.3236 | 0.2380 | a00000419 | [6] |
| | | 1005 | 1.1528 | 3.1265 | 3.0969 | 3.1303 | 0.6613 | a00000420 | |
| | | 1174 | 0.0505 | 0.0910 | 0.0902 | 0.0918 | 0.0412 | a00000421 | |
| 1.00 | 16.39 | 1115 | 0.2506 | 0.7473 | 0.7310 | 0.7495 | 0.2676 | a00000422 | [6] |
| | | 1063 | 1.2436 | 3.1065 | 2.9523 | 3.0279 | 1.3318 | a00000423* | |
| | | 1221 | 0.0739 | 0.1253 | 0.1254 | 0.1254 | 0.1167 | a00000439* | |
| 0.10 | 3.69 | 1108 | 0.3037 | 0.3078 | 0.3033 | 0.3056 | 0.2539 | a00000440 | [7] |
| | | 1014 | 1.2486 | 2.2990 | 2.0732 | 2.1424 | 0.9107 | a00000441* | |
| | | 1372 | 0.0410 | 0.0429 | 0.0432 | 0.0428 | 0.0420 | a00000427 | |
| 0.10 | 1.01 | 1162 | 0.1455 | 0.1111 | 0.1111 | 0.1113 | 0.1061 | a00000428 | [7] |
| | | 1007 | 0.5158 | 0.3540 | 0.3500 | 0.3523 | 0.3057 | ${a00000429} | |
| | | 1074 | 0.1147 | 0.1022 | 0.1001 | 0.1010 | 0.0707 | a00000430 | |
| 0.10 | 4.17 | 1022 | 0.4968 | 0.9257 | 0.8077 | 0.8444 | 0.1932 | a00000431* | [7] |
| | | 975 | 2.1530 | 10.4534 | 10.5319 | 10.4979 | 8.6371 | a00000432* | |
| | | 1113 | 0.3755 | 1.0117 | 0.9951 | 1.0064 | 0.4486 | a00000433* | |
| 0.10 | 17.78 | 1055 | 1.0493 | 4.2563 | 4.0069 | 4.0325 | 2.3928 | a00000434 | [7] |
| | | 1003 | 2.9324 | 14.6548 | 13.7606 | 13.7917 | 8.8267 | a00000435 | |

Table S3: Comparison of ignition-delay results for Mechanism1, Mechanism2, Mechanism3, and DynamicMech151203.

| **Equiv ratio Φ** | **P [atm]** | **T [K]** | $\tau_{\mathbf{ign}}$ **[ms]** | **Mech1 [ms]** | **Mech2 [ms]** | **Mech3 [ms]** | **Dynamic Mech [ms]** | **PrIMe ID** | **Ref** |
|---|---|---|---|---|---|---|---|---|---|
| | | 1608 | 0.0810 | 0.1121 | 0.1125 | 0.1126 | 0.1096 | a00000436 | |
| 0.10 | 0.94 | 1299 | 0.2626 | 0.3110 | 0.3118 | 0.3129 | 0.3044 | a00000437* | [7] |
| | | 1090 | 0.8520 | 0.9487 | 0.9445 | 0.9504 | 0.8847 | a00000438 | |
| | | 1192 | 0.1241 | 0.1439 | 0.1298 | 0.1330 | 0.0671 | a00000442 | |
| 0.10 | 16.31 | 1136 | 0.5109 | 1.5750 | 1.4266 | 1.4894 | 0.3127 | a00000443* | [7] |
| | | 1084 | 2.1028 | 7.2727 | 6.4609 | 6.5958 | 3.0409 | a00000444* | |
| | | 1534 | 0.0811 | 0.0702 | 0.0703 | 0.0699 | 0.0678 | a00000397 | |
| 0.50 | 0.99 | 1262 | 0.2668 | 0.2054 | 0.2071 | 0.2075 | 0.1997 | a00000398 | [7] |
| | | 1072 | 0.8779 | 0.6450 | 0.6468 | 0.6468 | 0.6013 | a00000399 | |
| | | 1183 | 0.0939 | 0.0925 | 0.0920 | 0.0926 | 0.0829 | a00000400 | |
| 0.50 | 4.08 | 1118 | 0.3172 | 0.1793 | 0.1774 | 0.1802 | 0.1436 | a00000401* | [7] |
| | | 1059 | 1.0718 | 0.6965 | 0.6833 | 0.6970 | 0.3286 | a00000402* | |
| | | 1192 | 0.1853 | 0.1801 | 0.1716 | 0.1767 | 0.0592 | a00000403 | |
| 0.50 | 15.57 | 1144 | 0.5729 | 0.8245 | 0.7407 | 0.7717 | 0.2880 | a00000404 | [7] |
| | | 1101 | 1.7710 | 2.5422 | 2.1622 | 2.2671 | 0.9766 | a00000405 | |
| | | 1623 | 0.0849 | 0.0611 | 0.0611 | 0.0611 | 0.0625 | a00000406* | |
| 3.99 | 1.06 | 1308 | 0.2522 | 0.2013 | 0.2014 | 0.2017 | 0.2034 | a00000407 | [7] |
| | | 1096 | 0.7491 | 0.6646 | 0.6626 | 0.6666 | 0.6550 | a00000408 | |
| | | 1297 | 0.0565 | 0.0590 | 0.0591 | 0.0589 | 0.0587 | a00000409 | |
| 3.99 | 3.98 | 1164 | 0.1954 | 0.1306 | 0.1306 | 0.1312 | 0.1244 | a00000410 | [7] |

Table S3: Comparison of ignition-delay results for Mechanism1, Mechanism2, Mechanism3, and DynamicMech151203.

| **Equiv ratio Φ** | **P [atm]** | **T [K]** | $\tau_{\mathbf{ign}}$ **[ms]** | **Mech1 [ms]** | **Mech2 [ms]** | **Mech3 [ms]** | **Dynamic Mech [ms]** | **PrIMe ID** | **Ref** |
|---|---|---|---|---|---|---|---|---|---|
| | | 1057 | 0.6756 | 0.4523 | 0.4513 | 0.4569 | 0.3392 | a00000411* | |
| | | 1143 | 0.1697 | 0.2319 | 0.2350 | 0.2398 | 0.1039 | a00000412 | |
| 3.99 | 14.87 | 1069 | 0.7237 | 1.6455 | 1.6456 | 1.7219 | 0.7081 | a00000413 | [7] |
| | | 1004 | 3.0870 | 8.6285 | 8.7015 | 8.9960 | 4.1206 | a00000414 | |
| | | 1009 | 0.2344 | 0.6922 | 0.6872 | 0.6961 | 0.1452 | a00000457 | |
| 0.42 | 3.28 | 972 | 0.8252 | 4.0392 | 4.0517 | 4.0382 | 2.4558 | a00000458* | [8] |
| | | 938 | 2.9051 | 14.3582 | 14.0180 | 13.9642 | 14.0914 | a00000459* | |
| | | 1062 | 0.3217 | 0.3889 | 0.3865 | 0.3902 | 0.3210 | a00000376 | |
| 1.00 | 3.56 | 1012 | 1.0194 | 1.2506 | 1.2431 | 1.2570 | 0.6748 | a00000377* | [8] |
| | | 966 | 3.2307 | 15.6339 | 15.6974 | 15.7585 | 6.5254 | a00000378* | |
| | | 1296 | 0.2278 | 0.3240 | 0.3266 | 0.3266 | 0.3198 | a00000466 | |
| 1.00 | 1.00 | 1184 | 0.3902 | 0.5702 | 0.5701 | 0.5700 | 0.5593 | a00000467 | [9] |
| | | 1089 | 0.6685 | 1.0229 | 1.0155 | 1.0192 | 0.9823 | a00000468 | |
| | | 1564 | 0.1707 | 0.3284 | 0.3261 | 0.3263 | 0.3292 | a00000472 | |
| 1.03 | 1.00 | 1411 | 0.3018 | 0.5864 | 0.5807 | 0.5857 | 0.5711 | a00000473 | [9] |
| | | 1286 | 0.5337 | 1.0302 | 1.0187 | 1.0205 | 0.9976 | a00000474* | |
| | | 1386 | 0.1634 | 0.2577 | 0.2605 | 0.2598 | 0.2589 | a00000469* | |
| 1.47 | 1.00 | 1280 | 0.2403 | 0.4156 | 0.4170 | 0.4168 | 0.4162 | a00000470* | [9] |
| | | 1190 | 0.3532 | 0.6628 | 0.6661 | 0.6676 | 0.6564 | a00000471* | |
| | | 1270 | 0.0263 | 0.0534 | 0.0529 | 0.0543 | 0.0323 | a00000361 | |

Table S3: Comparison of ignition-delay results for Mechanism1, Mechanism2, Mechanism3, and DynamicMech151203.

| **Equiv ratio Φ** | **P [atm]** | **T [K]** | $\tau_{\mathbf{ign}}$ **[ms]** | **Mech1 [ms]** | **Mech2 [ms]** | **Mech3 [ms]** | **Dynamic Mech [ms]** | **PrIMe ID** | **Ref** |
|---|---|---|---|---|---|---|---|---|---|
| 1.00 | 33.00 | 1242 | 0.0592 | 0.1064 | 0.1064 | 0.1093 | 0.0497 | a00000362 | [10] |
| | | 1215 | 0.1337 | 0.2175 | 0.2185 | 0.2253 | 0.0901 | a00000363 | |
| | | 1714 | 0.0235 | 0.0372 | 0.0370 | 0.0375 | 0.0369 | a00000364 | |
| 1.00 | 64.00 | 1578 | 0.0423 | 0.0597 | 0.0596 | 0.0600 | 0.0579 | a00000365 | [10] |
| | | 1461 | 0.0760 | 0.1069 | 0.1063 | 0.1083 | 0.0962 | a00000366 | |
| | | 1327 | 0.1031 | 0.1136 | 0.1154 | 0.1208 | 0.0644 | a00000367 | |
| 1.00 | 64.00 | 1311 | 0.1438 | 0.1549 | 0.1582 | 0.1681 | 0.0818 | a00000368* | [10] |
| | | 1295 | 0.2007 | 0.2172 | 0.2202 | 0.2372 | 0.1067 | a00000369* | |
| | | 1566 | 0.0668 | 0.1112 | 0.1125 | 0.1123 | 0.1077 | a00000424 | |
| 0.25 | 1.32 | 1365 | 0.1137 | 0.2230 | 0.2220 | 0.2232 | 0.2169 | a00000425 | [11] |
| | | 1210 | 0.1933 | 0.4531 | 0.4490 | 0.4501 | 0.4364 | a00000426* | |
| | | 1045 | 0.5000 | 0.7352 | 0.7328 | 0.7414 | 0.3524 | a00000379 | |
| 2.00 | 5.00 | 1016 | 1.3800 | 3.7181 | 3.7042 | 3.7514 | 0.9310 | a00000380 | [12] |
| | | 990 | 3.8100 | 11.8584 | 11.8627 | 12.1387 | 3.7999 | a00000381 | |

* Indicates target was not included in final, reduced dataset.

Table S4: $\ell_2$-norm of the difference between each mechanisms prediction, $M(x)$, to the measured ignition delay, $\tau_{\text{ign}}$.

| | $\|\|M(x) - \tau_{\mathbf{ign}}\|\|_2$ |
|---:|:---:|
| **Mechanism 1** | 29.395 |
| **Mechanism 2** | 28.775 |
| **Mechanism 3** | 29.086 |
| **DynamicMech151203** | 15.800 |

## References


[1] T. Asaba, W. Gardiner, R. Stubbeman, Shock-tube study of the hydrogen-oxygen reaction, in: Symposium (International) on Combustion, Vol. 10, Elsevier, 1965, pp. 295–302. `doi:10.1016/S0082-0784(65)80175-8`.

[2] N. Chaumeix, S. Pichon, F. Lafosse, C. Paillard, Role of chemical kinetics on the detonation properties of hydrogen/natural gas/air mixtures, International Journal of Hydrogen Energy 32 (13) (2007) 2216–2226. `doi:10.1016/j.ijhydene.2007.04.008`.

[3] R. Cheng, A. Oppenheim, Autoignition in methane hydrogen mixtures, Combustion and Flame 58 (2) (1984) 125–139. `doi:10.1016/0010-2180(84)90088-9`.

[4] A. Cohen, J. Larsen, Brl report no. 1386, Ballistics Research Laboratories, Aberdeen, Maryland.

[5] S. Fujimoto, M. Suzuki, The induction period of hydrogenoxygen and methane-oxygen mixtures in a shock tube, Memoirs Defense Academy, Japan 8 (3) (1967) 1037–1046.

[6] J. Herzler, C. Naumann, Shock-tube study of the ignition of methane/ethane/hydrogen mixtures with hydrogen contents from 0% to 100% at different pressures, Proceedings of the combustion institute 32 (1) (2009) 213–220. `doi:10.1016/j.proci.2008.07.034`.

[7] C. Naumann, J. Herzler, P. Griebel, H. Curran, A. Kéromnès, I. Mantzaras, Results of ignition delay times for hydrogen-rich and syngas fuel mixtures measured, Deliverable 1.1.3, H2-IGCC.

[8] G. Pang, D. Davidson, R. Hanson, Experimental study and modeling of shock tube ignition delay times for hydrogen–oxygen–argon mixtures at low temperatures, Proceedings of the combustion institute 32 (1) (2009) 181–188. doi:10.1016/j.proci.2008.06.014.

[9] E. Petersen, D. Kalitan, M. Rickard, Chemical kinetics of OH* chemiluminescence in high-temperature reacting flows, in: Proceedings of the Joint Meeting of the US Sections of the Combustion Institute, Vol. 3, 2003.

[10] E. Petersen, D. Davidson, M. Roehrig, R. Hanson, Shock-induced ignition of high-pressure $H_2$-$O_2$-Ar and $CH_4$-$O_2$-Ar mixtures, in: AIAA, ASME, SAE, and ASEE, Joint Propulsion Conference and Exhibit, 31 st, San Diego, CA, 1995.

[11] G. Schott, J. Kinsey, Kinetic studies of hydroxyl radicals in shock waves. II. Induction times in the hydrogen-oxygen reaction, The Journal of Chemical Physics 29 (5) (1958) 1177–1182. doi:10.1063/1.1744674.

[12] G. B. Skinner, G. H. Ringrose, Ignition delays of a Hydrogen—Oxygen—Argon mixture at relatively low temperatures, The Journal of Chemical Physics 42 (6) (1965) 2190–2192. doi:10.1063/1.1696266.

[13] S. Tse, D. Zhu, C. Law, Morphology and burning rates of expanding spherical flames in $H_2$/$O_2$/inert mixtures up to 60 atmospheres, Proceedings of the Combustion Institute 28 (2) (2000) 1793–1800. doi:10.1016/S0082-0784(00)80581-0.

[14] M. P. Burke, M. Chaos, F. L. Dryer, Y. Ju, Negative pressure dependence of mass burning rates of $H_2$/CO/$O_2$/diluent flames at low flame temperatures, Combustion and Flame 157 (4) (2010) 618–631. doi:10.1016/j.combustflame.2009.08.009.

## 3. Flame Simulations

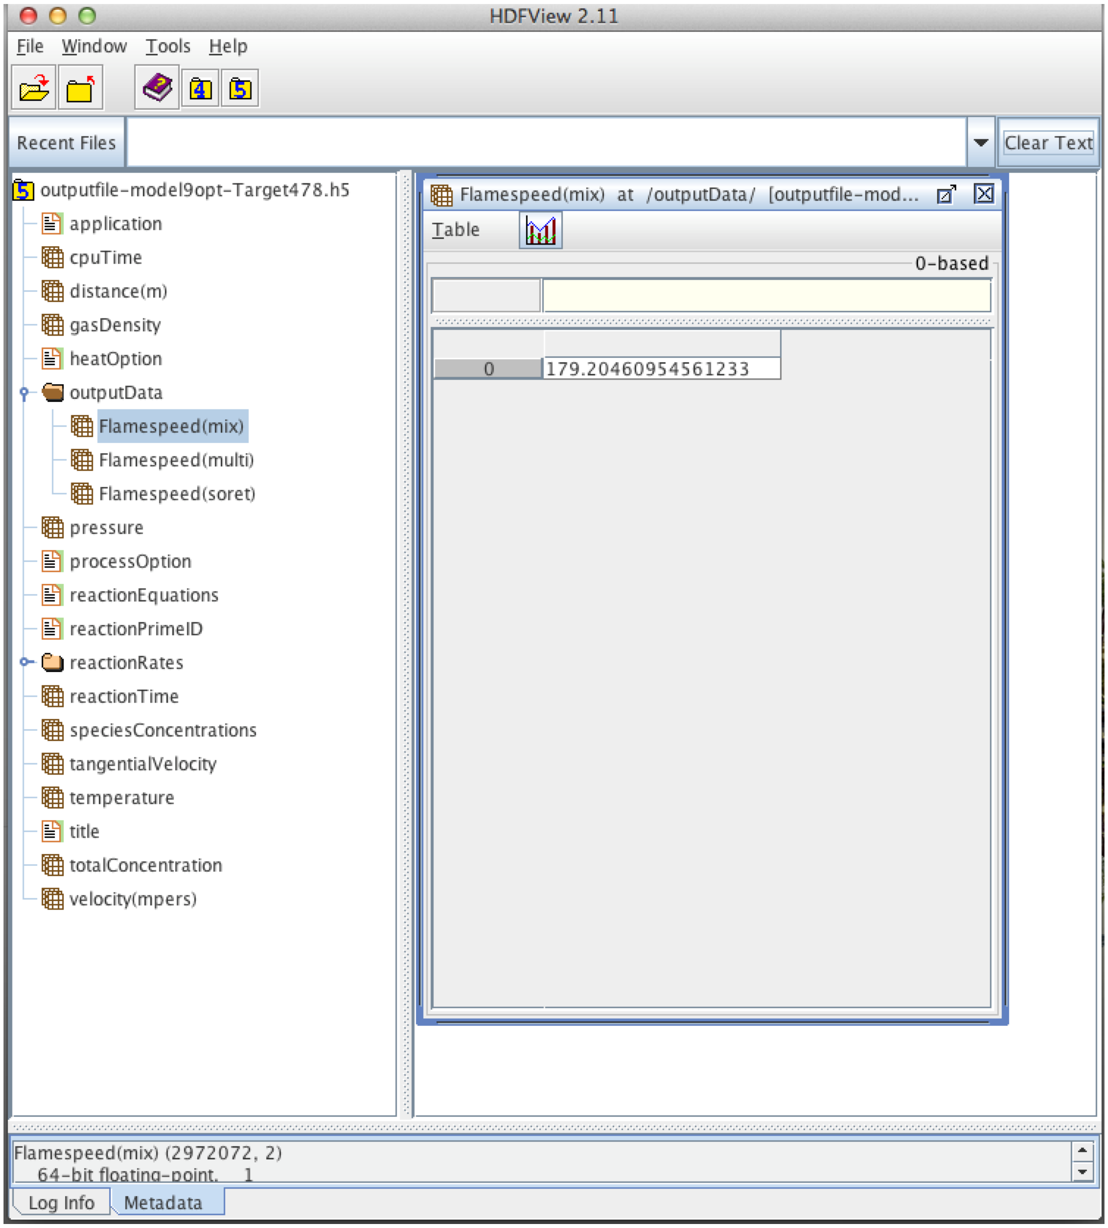


Figure S4: Screenshot of HDF5 simulation output for calculated flame speed.

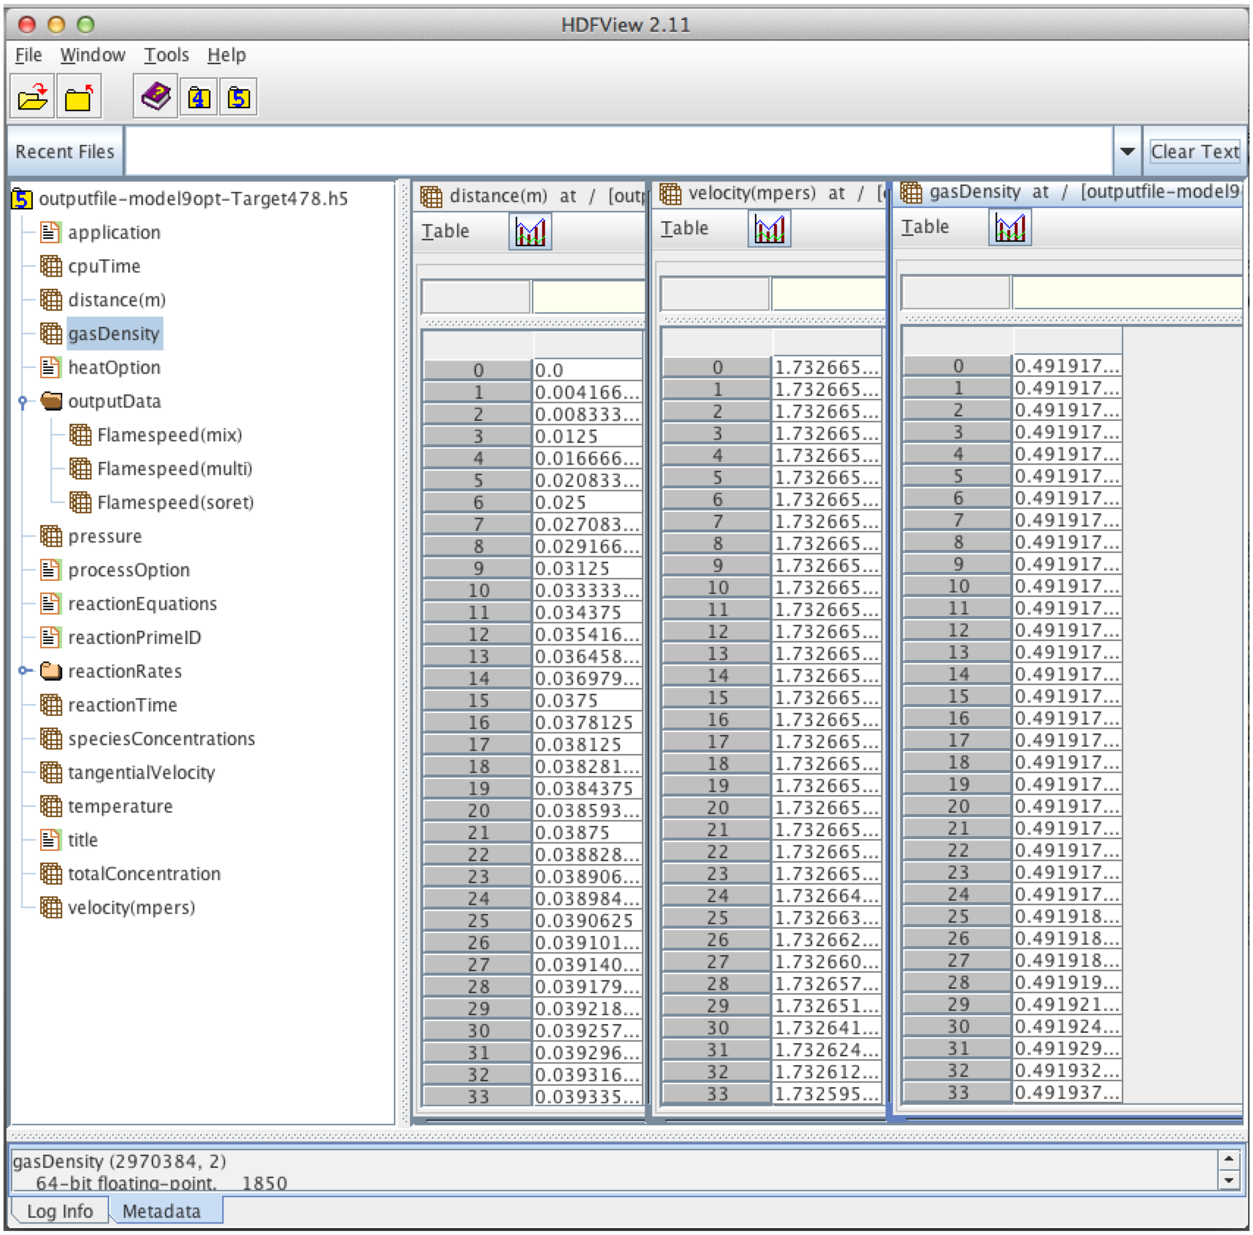


| | distance(m) | velocity(mpers) | gasDensity |
|---|---|---|---|
| 0 | 0.0 | 1.732665... | 0.491917... |
| 1 | 0.004166... | 1.732665... | 0.491917... |
| 2 | 0.008333... | 1.732665... | 0.491917... |
| 3 | 0.0125 | 1.732665... | 0.491917... |
| 4 | 0.016666... | 1.732665... | 0.491917... |
| 5 | 0.020833... | 1.732665... | 0.491917... |
| 6 | 0.025 | 1.732665... | 0.491917... |
| 7 | 0.027083... | 1.732665... | 0.491917... |
| 8 | 0.029166... | 1.732665... | 0.491917... |
| 9 | 0.03125 | 1.732665... | 0.491917... |
| 10 | 0.033333... | 1.732665... | 0.491917... |
| 11 | 0.034375 | 1.732665... | 0.491917... |
| 12 | 0.035416... | 1.732665... | 0.491917... |
| 13 | 0.036458... | 1.732665... | 0.491917... |
| 14 | 0.036979... | 1.732665... | 0.491917... |
| 15 | 0.0375 | 1.732665... | 0.491917... |
| 16 | 0.0378125 | 1.732665... | 0.491917... |
| 17 | 0.038125 | 1.732665... | 0.491917... |
| 18 | 0.038281... | 1.732665... | 0.491917... |
| 19 | 0.0384375 | 1.732665... | 0.491917... |
| 20 | 0.038593... | 1.732665... | 0.491917... |
| 21 | 0.03875 | 1.732665... | 0.491917... |
| 22 | 0.038828... | 1.732665... | 0.491917... |
| 23 | 0.038906... | 1.732665... | 0.491917... |
| 24 | 0.038984... | 1.732664... | 0.491917... |
| 25 | 0.0390625 | 1.732663... | 0.491918... |
| 26 | 0.039101... | 1.732662... | 0.491918... |
| 27 | 0.039140... | 1.732660... | 0.491918... |
| 28 | 0.039179... | 1.732657... | 0.491919... |
| 29 | 0.039218... | 1.732651... | 0.491921... |
| 30 | 0.039257... | 1.732641... | 0.491924... |
| 31 | 0.039296... | 1.732624... | 0.491929... |
| 32 | 0.039316... | 1.732612... | 0.491932... |
| 33 | 0.039335... | 1.732595... | 0.491937... |

Figure S5: Screenshot of HDF5 simulation output for distance, velocity, and density details.

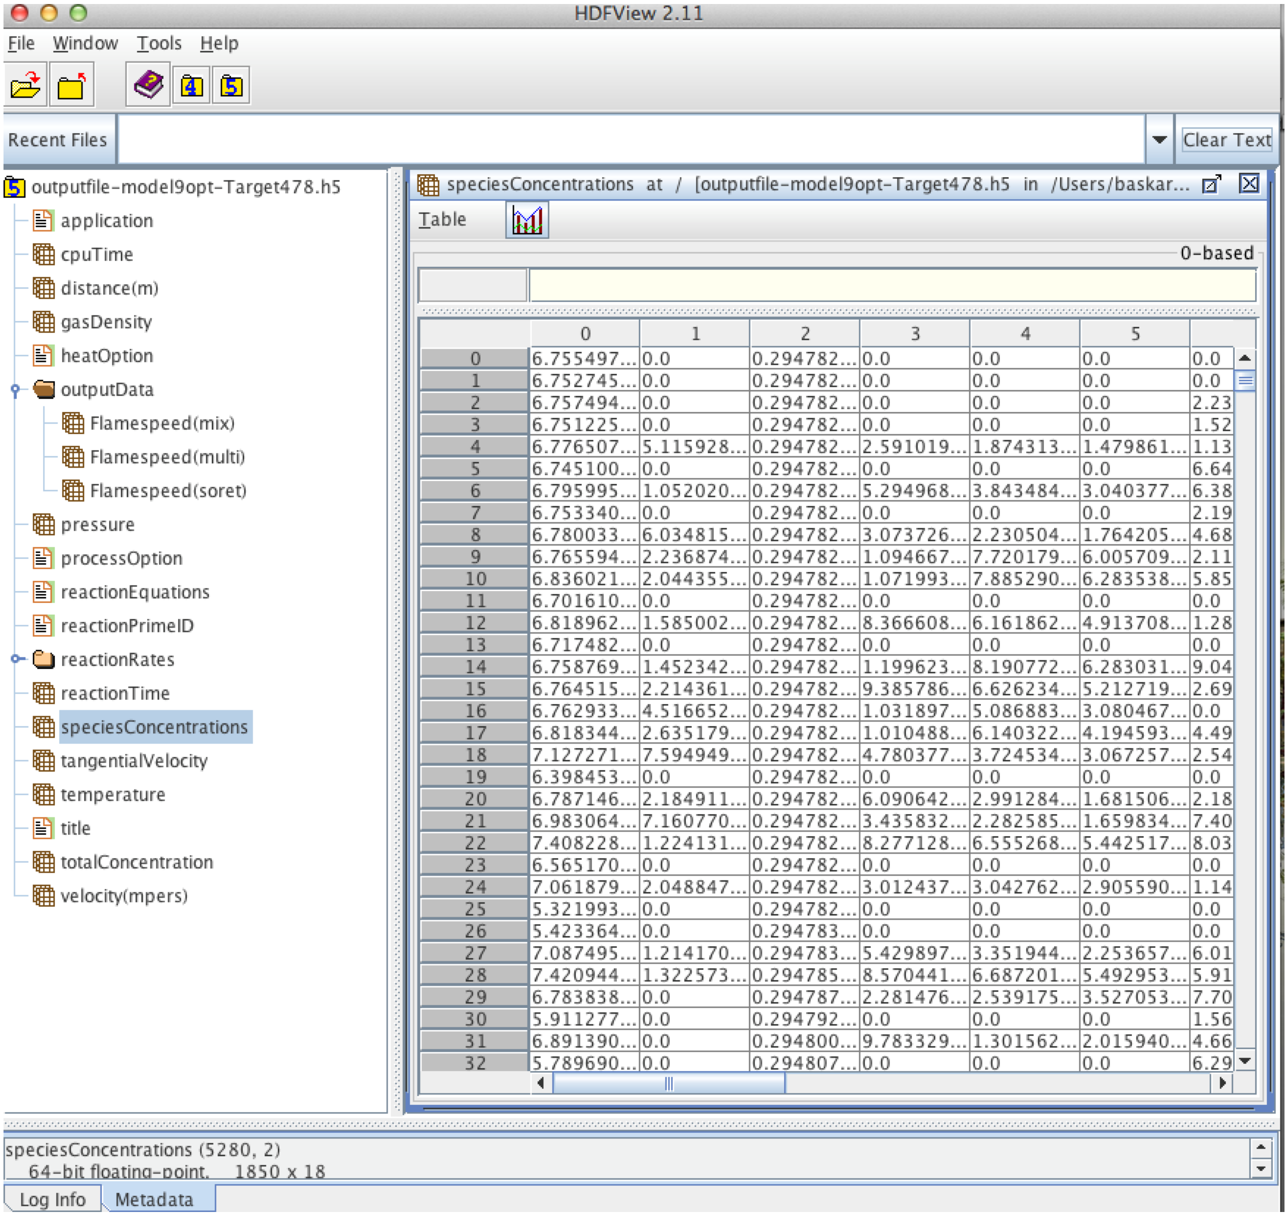


Figure S6: Screenshot of HDF5 simulation output for species concentrations.

Table S5: Comparison of flame-speed results (multicomponent transport with Soret effect) for Mechanism1, Mechanism2, Mechanism3, and DynamicMech151203.

| **Target PrIMe ID** | **Preferred Key** | **Pressure [atm]** | $\Phi$ | **Measured [cm/s]** | **Mech1 [cm/s]** | **Mech2 [cm/s]** | **Mech3 [cm/s]** | **DynamicMech [cm/s]** |
|---|---|---|---|---|---|---|---|---|
| a00000476 | H2 F - 476 | 1 | 0.6 | 81.88 | 83.94 | 88.87 | 86.39 | 97.95 |
| a00000477 | H2 F - 477 | 1 | 1.65 | 280.21 | 280.28 | 284.83 | 280.84 | 286.38 |
| a00000478 | H2 F - 478 | 1 | 4 | 165.29 | 162.10 | 165.37 | 160.18 | 173.27 |
| a00000479 | H2 F - 479 | 20 | 1.5 | 80.9 | 76.84 | 81.72 | 75.67 | 106.17 |
| a00000480 | H2 F - 480 | 20 | 2 | 64.05 | 59.42 | 63.17 | 56.14 | 90.05 |
| a00000481 | H2 F - 481 | 20 | 0.85 | 18.35 | 24.29 | 27.91 | 26.28 | 43.49 |
| a00000482 | H2 F - 482 | 15 | 0.85 | 26.9 | 33.30 | 37.23 | 35.32 | 53.22 |
| a00000483 | H2 F - 483 | 10 | 0.85 | 45.3 | 46.28 | 50.34 | 48.08 | 65.91 |
| a00000484 | H2 F - 484 | 14 | 2.5 | 28.7 | 30.32 | 32.14 | 27.84 | 48.31 |
| a00000485 | H2 F - 485 | 25 | 2.5 | 27.7 | 32.04 | 34.16 | 29.28 | 53.54 |

Table S6: Comparison of flame speed results (mixture-averaged transport) with CloudFlame-Cantera and CHEMKIN-PRO for Mechanism1.

| **Target PrIMe ID** | **Preferred Key** | **Pressure [atm]** | $\Phi$ | **Mechanism1 CLOUDFLAME-CANTERA [cm/s]** | **Mechanism1 CHEMKIN PRO [cm/s]** |
|---|---|---|---|---|---|
| a00000476 | H2 F - 476 | 1 | 0.6 | 117.41 | 117.86 |
| a00000477 | H2 F - 477 | 1 | 1.65 | 324.76 | 329.36 |
| a00000478 | H2 F - 478 | 1 | 4 | 125.08 | 126.03 |
| a00000479 | H2 F - 479 | 20 | 1.5 | 94.83 | 94.59 |
| a00000480 | H2 F - 480 | 20 | 2 | 73.74 | 73.29 |
| a00000481 | H2 F - 481 | 20 | 0.85 | 36.76 | 36.79 |
| a00000482 | H2 F - 482 | 15 | 0.85 | 47.32 | 47.30 |
| a00000483 | H2 F - 483 | 10 | 0.85 | 61.58 | 61.57 |
| a00000484 | H2 F - 484 | 14 | 2.5 | 38.16 | 37.95 |
| a00000485 | H2 F - 485 | 25 | 2.5 | 37.84 | 37.61 |

## 4. Consistency Analysis

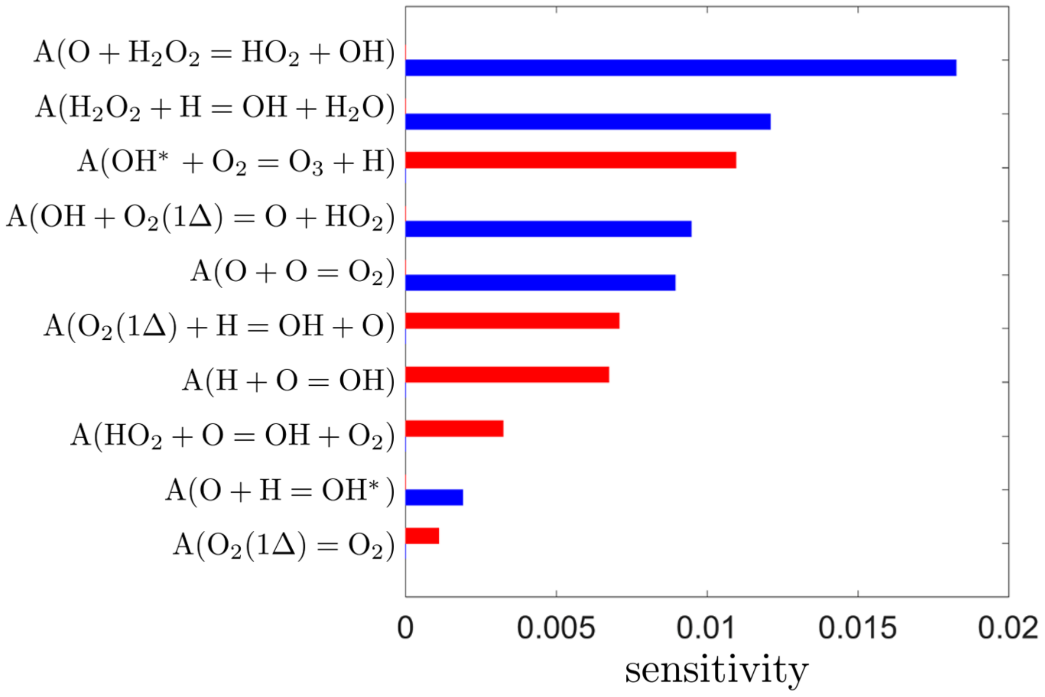


Figure S7: Normalized sensitivity of the consistency measure with respect to parameter bounds. Blue bars indicate sensitivity to a parameters lower bound ($L_e$), and red bars are upper bounds ($U_e$), where $e$ is the parameter index. Sensitivities of the consistency measure to the experimental bounds shown in Figure 2 in the paper are an order of magnitude larger than those of the parameter bounds. Therefore, we examined the experimental bounds to resolve the inconsistency.

.

## 5. Cantera Input

### *5.1. Mechanism1 - m00000007.cti*

```
#-------------------------------------------------------------------------------

#HDF5
# CTI Generated : 2017-12-02 01:04:44
#-------------------------------------------------------------------------------


units(length='cm', time='s', quantity='mol', act_energy='cal/mol')


ideal_gas(name='gas',
          elements="Ar C H He N O",
          species="""Ar He N2 C(GR) CO
                     CO2 H H2 O O2
                     OH H2O HO2 H2O2""",
          reactions='all',
          initial_state=state(temperature= 298.15, pressure=
              100000.0))

#-------------------------------------------------------------------------------

#Species data
#-------------------------------------------------------------------------------


species(name='Ar',
        atoms='Ar:1',
        thermo=(NASA([300.0, 1000.0],
                     [2.5, 0.0, 0.0,
                      0.0, 0.0, -745.375,
                      4.366001]),
                NASA([1000.0, 5000.0],
                     [2.5, 0.0, 0.0,
                      0.0, 0.0, -745.375,
                      4.366001])),
        transport = gas_transport(
                geom = "atom",
```

```
              well_depth = 136.5,
              diam = 3.33))

species(name='He',
        atoms='He:1',
        thermo=(NASA([300.0, 1000.0],
                   [2.5, 0.0, 0.0,
                    0.0, 0.0, -745.375,
                    0.9153488]),
              NASA([1000.0, 5000.0],
                   [2.5, 0.0, 0.0,
                    0.0, 0.0, -745.375,
                    0.9153488])),
        transport = gas_transport(
              geom = "atom",
              well_depth = 10.2,
              diam = 2.576))

species(name='N2',
        atoms='N:2',
        thermo=(NASA([300.0, 1000.0],
                   [3.298677, 0.00140824, -3.96322e-06,
                    5.64152e-09, -2.44486e-12, -1020.9,
                    3.950372]),
              NASA([1000.0, 5000.0],
                   [2.92664, 0.001487977, -5.68476e-07,
                    1.0097e-10, -6.75335e-15, -922.7977,
                    5.980528])),
        transport = gas_transport(
              geom = "linear",
              well_depth = 97.53,
              diam = 3.621,
              polar = 1.76,
              rot_relax = 4.0))

species(name='C(GR)',
        atoms='C:1',
        thermo=(NASA([200.0, 1000.0],
                   [-0.31087, 0.0044035, 1.9039e-06,
                    -6.3855e-09, 2.9896e-12, -108.6508,
```

```
                1.1138]),
            NASA([1000.0, 5000.0],
                [1.4557, 0.0017171, -6.9758e-07,
                 1.3528e-10, -9.6765e-15, -695.128,
                 -8.5257])),
    transport = gas_transport(
            geom = "atom",
            well_depth = 71.4,
            diam = 3.298))

species(name='CO',
    atoms='C:1 O:1',
    thermo=(NASA([300.0, 1000.0],
                [3.262452, 0.001511941, -3.88176e-06,
                 5.58194e-09, -2.47495e-12, -14310.54,
                 4.848897]),
            NASA([1000.0, 5000.0],
                [3.025078, 0.001442689, -5.63083e-07,
                 1.01858e-10, -6.91095e-15, -14268.35,
                 6.108218])),
    transport = gas_transport(
            geom = "linear",
            well_depth = 98.1,
            diam = 3.65,
            polar = 1.95,
            rot_relax = 1.8))

species(name='CO2',
    atoms='C:1 O:2',
    thermo=(NASA([300.0, 1000.0],
                [2.275725, 0.009922072, -1.04091e-05,
                 6.86669e-09, -2.11728e-12, -48373.14,
                 10.18849]),
            NASA([1000.0, 5000.0],
                [4.453623, 0.003140169, -1.27841e-06,
                 2.394e-10, -1.66903e-14, -48966.96,
                 -0.9553959])),
    transport = gas_transport(
            geom = "linear",
            well_depth = 244.0,
```

```
                diam = 3.763,
                polar = 2.65,
                rot_relax = 2.1))

species(name='H',
        atoms='H:1',
        thermo=(NASA([300.0, 1000.0],
                     [2.5, 0.0, 0.0,
                      0.0, 0.0, 25471.63,
                      -0.4601176]),
                NASA([1000.0, 5000.0],
                     [2.5, 0.0, 0.0,
                      0.0, 0.0, 25471.63,
                      -0.4601176])),
        transport = gas_transport(
                geom = "atom",
                well_depth = 145.0,
                diam = 2.05))

species(name='H2',
        atoms='H:2',
        thermo=(NASA([300.0, 1000.0],
                     [3.298124, 0.000824944, -8.14302e-07,
                      -9.47543e-11, 4.13487e-13, -1012.521,
                      -3.294094]),
                NASA([1000.0, 5000.0],
                     [2.991423, 0.000700064, -5.63383e-08,
                      -9.23158e-12, 1.58275e-15, -835.034,
                      -1.35511])),
        transport = gas_transport(
                geom = "linear",
                well_depth = 38.0,
                diam = 2.92,
                polar = 0.79,
                rot_relax = 280.0))

species(name='O',
        atoms='O:1',
        thermo=(NASA([300.0, 1000.0],
                     [2.946429, -0.001638166, 2.42103e-06,
```

```
                    -1.60284e-09, 3.8907e-13, 29147.64,
                    2.963995]),
              NASA([1000.0, 5000.0],
                   [2.54206, -2.75506e-05, -3.1028e-09,
                    4.55107e-12, -4.36805e-16, 29230.8,
                    4.920308])),
        transport = gas_transport(
              geom = "atom",
              well_depth = 80.0,
              diam = 2.75))

species(name='O2',
        atoms='O:2',
        thermo=(NASA([300.0, 1000.0],
                   [3.212936, 0.001127486, -5.75615e-07,
                    1.31388e-09, -8.76855e-13, -1005.249,
                    6.034738]),
              NASA([1000.0, 5000.0],
                   [3.697578, 0.00061352, -1.25884e-07,
                    1.77528e-11, -1.13644e-15, -1233.93,
                    3.189166])),
        transport = gas_transport(
              geom = "linear",
              well_depth = 107.4,
              diam = 3.458,
              polar = 1.6,
              rot_relax = 3.8))

species(name='OH',
        atoms='H:1 O:1',
        thermo=(NASA([200.0, 1000.0],
                   [4.12530561, -0.003225449, 6.52765e-06,
                    -5.79854e-09, 2.06237e-12, 3346.30913,
                    -0.69043296]),
              NASA([1000.0, 6000.0],
                   [2.86472886, 0.001056504, -2.59083e-07,
                    3.05219e-11, -1.33196e-15, 3683.62875,
                    5.70164073])),
        transport = gas_transport(
              geom = "linear",
```

```
            well_depth = 80.0,
            diam = 2.75))

species(name='H2O',
        atoms='H:2 O:1',
        thermo=(NASA([300.0, 1000.0],
                     [3.386842, 0.003474982, -6.3547e-06,
                      6.96858e-09, -2.50659e-12, -30208.11,
                      2.590233]),
                NASA([1000.0, 5000.0],
                     [2.672146, 0.003056293, -8.73026e-07,
                      1.201e-10, -6.39162e-15, -29899.21,
                      6.862817])),
        transport = gas_transport(
                geom = "nonlinear",
                well_depth = 572.4,
                diam = 2.605,
                dipole = 1.844,
                rot_relax = 4.0))

species(name='HO2',
        atoms='H:1 O:2',
        thermo=(NASA([200.0, 1000.0],
                     [4.30179801, -0.004749121, 2.11583e-05,
                      -2.42764e-08, 9.29225e-12, 294.80804,
                      3.71666245]),
                NASA([1000.0, 3500.0],
                     [4.0172109, 0.00223982, -6.33658e-07,
                      1.14246e-10, -1.07909e-14, 111.856713,
                      3.78510215])),
        transport = gas_transport(
                geom = "nonlinear",
                well_depth = 107.4,
                diam = 3.458,
                rot_relax = 1.0))

species(name='H2O2',
        atoms='H:2 O:2',
        thermo=(NASA([300.0, 1000.0],
                     [3.388754, 0.006569226, -1.48501e-07,
```

```
                  -4.62581e-09, 2.47152e-12, -17663.15,
                  6.785363]),
             NASA([1000.0, 5000.0],
                 [4.573167, 0.004336136, -1.47469e-06,
                  2.3489e-10, -1.43165e-14, -18006.96,
                  0.501137])),
       transport = gas_transport(
             geom = "nonlinear",
             well_depth = 107.4,
             diam = 3.458,
             rot_relax = 3.8))


#--------------------------------------------------------------------------------

#Reaction data
#--------------------------------------------------------------------------------


#Reaction 1:
reaction('O2 + H <=> OH + O', [1.04e+14, 0.0, 15309.835])

#Reaction 2:
reaction('H2 + O <=> OH + H', [8.7923244e+14, 0.0, 19174.55],
        options='duplicate')

#Reaction 3:
reaction('H2 + O <=> OH + H', [3.81803676e+12, 0.0, 7948.0],
        options='duplicate')

#Reaction 4:
reaction('H2 + OH <=> H2O + H', [216194826.0, 1.51, 3429.562])

#Reaction 5:
reaction('OH + OH <=> H2O + O', [33483.0984, 2.42, -1927.39])

#Reaction 6:
three_body_reaction('H + H + M <=> H2 + M', [3.143e+20, -1.806,
   982.555066967],
        efficiencies='H2:2.5 H2O:12.0 CO:1.9 CO2:3.8 Ar:0.0 He:0.0
```

```
            ')

#Reaction 7:
reaction('H + H + Ar <=> H2 + Ar', [4.011e+19, -1.506,
    982.555066967])

#Reaction 8:
reaction('H + H + He <=> H2 + He', [4.011e+19, -1.506,
    982.555066967])

#Reaction 9:
three_body_reaction('O + O + M <=> O2 + M', [6.16524893053e+15,
    -0.5, 0.0],
        efficiencies='H2:2.53 H2O:11.76 CO:1.88 CO2:3.82 Ar:0.0 He
            :0.0 ')

#Reaction 10:
reaction('O + O + Ar <=> O2 + Ar', [1.88584084934e+13, 0.0,
    -1788.3])

#Reaction 11:
reaction('O + O + He <=> O2 + He', [1.88584084934e+13, 0.0,
    -1788.3])

#Reaction 12:
three_body_reaction('H + O + M <=> OH + M', [4.71460212335e+18,
    -1.0, 0.0],
        efficiencies='H2:2.54 H2O:12.31 CO:1.92 CO2:3.77 He:0.75 Ar
            :0.75 ')

#Reaction 13:
three_body_reaction('OH + H + M <=> H2O + M', [1.483e+28, -3.798,
    2706.52897774],
        efficiencies='H2:3.0 O2:1.5 N2:2.0 He:1.1 CO:1.9 CO2:3.8
            H2O:0.0 ')

#Reaction 14:
reaction('OH + H + H2O <=> H2O + H2O', [2.46e+26, -2.916,
    2096.18418054])
```

```
#Reaction 15:
falloff_reaction('O2 + H (+ M) <=> HO2 (+ M)',
               kf=[4.65e+12, 0.44, 0.0],
               kf0=[6.37e+20, -1.72, 524.568],
               efficiencies='H2:1.99 O2:0.78 H2O:14.0 CO:1.9 CO2
                   :3.8 Ar:0.67 He:0.8 ',
        falloff = Troe(A = 0.5, T3 = 1e-30, T1 = 1e+30, T2 = 0))

#Reaction 16:
reaction('O2 + H2 <=> HO2 + H', [1341000.0, 2.314, 53420.1782336])

#Reaction 17:
reaction('HO2 + H <=> OH + OH', [7.08e+13, 0.0, 300.169572393])

#Reaction 18:
reaction('HO2 + O <=> OH + O2', [28500000000.0, 1.0,
   -724.309178184])

#Reaction 19:
reaction('O2 + H2O <=> HO2 + OH', [3.956e+13, 0.294,
   69070.0191729])

#Reaction 20:
reaction('HO2 + HO2 <=> H2O2 + O2', [4.2e+14, 0.0, 11981.61],
        options='duplicate')

#Reaction 21:
reaction('HO2 + HO2 <=> H2O2 + O2', [130000000000.0, 0.0,
   -1629.34],
        options='duplicate')

#Reaction 22:
falloff_reaction('OH + OH (+ M) <=> H2O2 (+ M)',
               kf=[45280000.0, 1.657, -1818.02704346],
               kf0=[5.637e+19, -1.543, -1818.02704346],
               efficiencies='H2:3.7 H2O:7.5 O2:1.2 H2O2:7.7 N2:1.5
                   He:0.65 CO:2.8 CO2:1.6 ',
        falloff = Troe(A = 0.43, T3 = 1e-30, T1 = 1e+30, T2 = 0))

#Reaction 23:
```

```
reaction('H2O2 + H <=> OH + H2O', [2.408856e+13, 0.0, 3974.0])

#Reaction 24:
reaction('H2O2 + H <=> H2 + HO2', [4.817712e+13, 0.0, 7948.0])

#Reaction 25:
reaction('O + H2O2 <=> HO2 + OH', [9635424.0, 2.0, 3974.0])

#Reaction 26:
reaction('OH + H2O2 <=> HO2 + H2O', [1.7378e+12, 0.0, 317.92],
        options='duplicate')

#Reaction 27:
reaction('OH + H2O2 <=> HO2 + H2O', [7.5858e+13, 0.0, 7272.42],
        options='duplicate')
```

*5.2. Mechanism2 - m00000008.cti*

```
#-------------------------------------------------------------------------------

#HDF5
# CTI Generated : 2017-12-02 01:05:27
#-------------------------------------------------------------------------------


units(length='cm', time='s', quantity='mol', act_energy='cal/mol')


ideal_gas(name='gas',
         elements="Ar C H He N O",
         species="""Ar He N2 C(GR) CO
                   CO2 H H2 O O2
                   OH H2O HO2 H2O2""",
         reactions='all',
         initial_state=state(temperature= 298.15, pressure=
             100000.0))

#-------------------------------------------------------------------------------

#Species data
#-------------------------------------------------------------------------------


species(name='Ar',
       atoms='Ar:1',
       thermo=(NASA([300.0, 1000.0],
                   [2.5, 0.0, 0.0,
                    0.0, 0.0, -745.375,
                    4.366001]),
              NASA([1000.0, 5000.0],
                   [2.5, 0.0, 0.0,
                    0.0, 0.0, -745.375,
                    4.366001])),
       transport = gas_transport(
              geom = "atom",
              well_depth = 136.5,
              diam = 3.33))
```

```
species(name='He',
        atoms='He:1',
        thermo=(NASA([300.0, 1000.0],
                     [2.5, 0.0, 0.0,
                      0.0, 0.0, -745.375,
                      0.9153488]),
                NASA([1000.0, 5000.0],
                     [2.5, 0.0, 0.0,
                      0.0, 0.0, -745.375,
                      0.9153488])),
        transport = gas_transport(
                geom = "atom",
                well_depth = 10.2,
                diam = 2.576))

species(name='N2',
        atoms='N:2',
        thermo=(NASA([300.0, 1000.0],
                     [3.298677, 0.00140824, -3.96322e-06,
                      5.64152e-09, -2.44486e-12, -1020.9,
                      3.950372]),
                NASA([1000.0, 5000.0],
                     [2.92664, 0.001487977, -5.68476e-07,
                      1.0097e-10, -6.75335e-15, -922.7977,
                      5.980528])),
        transport = gas_transport(
                geom = "linear",
                well_depth = 97.53,
                diam = 3.621,
                polar = 1.76,
                rot_relax = 4.0))

species(name='C(GR)',
        atoms='C:1',
        thermo=(NASA([200.0, 1000.0],
                     [-0.31087, 0.0044035, 1.9039e-06,
                      -6.3855e-09, 2.9896e-12, -108.6508,
                      1.1138]),
                NASA([1000.0, 5000.0],
```

```
                [1.4557, 0.0017171, -6.9758e-07,
                 1.3528e-10, -9.6765e-15, -695.128,
                 -8.5257])),
        transport = gas_transport(
                geom = "atom",
                well_depth = 71.4,
                diam = 3.298))

species(name='CO',
        atoms='C:1 O:1',
        thermo=(NASA([300.0, 1000.0],
                [3.262452, 0.001511941, -3.88176e-06,
                 5.58194e-09, -2.47495e-12, -14310.54,
                 4.848897]),
                NASA([1000.0, 5000.0],
                [3.025078, 0.001442689, -5.63083e-07,
                 1.01858e-10, -6.91095e-15, -14268.35,
                 6.108218])),
        transport = gas_transport(
                geom = "linear",
                well_depth = 98.1,
                diam = 3.65,
                polar = 1.95,
                rot_relax = 1.8))

species(name='CO2',
        atoms='C:1 O:2',
        thermo=(NASA([300.0, 1000.0],
                [2.275725, 0.009922072, -1.04091e-05,
                 6.86669e-09, -2.11728e-12, -48373.14,
                 10.18849]),
                NASA([1000.0, 5000.0],
                [4.453623, 0.003140169, -1.27841e-06,
                 2.394e-10, -1.66903e-14, -48966.96,
                 -0.9553959])),
        transport = gas_transport(
                geom = "linear",
                well_depth = 244.0,
                diam = 3.763,
                polar = 2.65,
```

```
                rot_relax = 2.1))

species(name='H',
        atoms='H:1',
        thermo=(NASA([300.0, 1000.0],
                     [2.5, 0.0, 0.0,
                      0.0, 0.0, 25471.63,
                      -0.4601176]),
                NASA([1000.0, 5000.0],
                     [2.5, 0.0, 0.0,
                      0.0, 0.0, 25471.63,
                      -0.4601176])),
        transport = gas_transport(
                geom = "atom",
                well_depth = 145.0,
                diam = 2.05))

species(name='H2',
        atoms='H:2',
        thermo=(NASA([300.0, 1000.0],
                     [3.298124, 0.000824944, -8.14302e-07,
                      -9.47543e-11, 4.13487e-13, -1012.521,
                      -3.294094]),
                NASA([1000.0, 5000.0],
                     [2.991423, 0.000700064, -5.63383e-08,
                      -9.23158e-12, 1.58275e-15, -835.034,
                      -1.35511])),
        transport = gas_transport(
                geom = "linear",
                well_depth = 38.0,
                diam = 2.92,
                polar = 0.79,
                rot_relax = 280.0))

species(name='O',
        atoms='O:1',
        thermo=(NASA([300.0, 1000.0],
                     [2.946429, -0.001638166, 2.42103e-06,
                      -1.60284e-09, 3.8907e-13, 29147.64,
                      2.963995]),
```

```
            NASA([1000.0, 5000.0],
                 [2.54206, -2.75506e-05, -3.1028e-09,
                  4.55107e-12, -4.36805e-16, 29230.8,
                  4.920308])),
        transport = gas_transport(
            geom = "atom",
            well_depth = 80.0,
            diam = 2.75))

species(name='O2',
        atoms='O:2',
        thermo=(NASA([300.0, 1000.0],
                 [3.212936, 0.001127486, -5.75615e-07,
                  1.31388e-09, -8.76855e-13, -1005.249,
                  6.034738]),
            NASA([1000.0, 5000.0],
                 [3.697578, 0.00061352, -1.25884e-07,
                  1.77528e-11, -1.13644e-15, -1233.93,
                  3.189166])),
        transport = gas_transport(
            geom = "linear",
            well_depth = 107.4,
            diam = 3.458,
            polar = 1.6,
            rot_relax = 3.8))

species(name='OH',
        atoms='H:1 O:1',
        thermo=(NASA([200.0, 1000.0],
                 [4.12530561, -0.003225449, 6.52765e-06,
                  -5.79854e-09, 2.06237e-12, 3346.30913,
                  -0.69043296]),
            NASA([1000.0, 6000.0],
                 [2.86472886, 0.001056504, -2.59083e-07,
                  3.05219e-11, -1.33196e-15, 3683.62875,
                  5.70164073])),
        transport = gas_transport(
            geom = "linear",
            well_depth = 80.0,
            diam = 2.75))
```

```
species(name='H2O',
        atoms='H:2 O:1',
        thermo=(NASA([300.0, 1000.0],
                     [3.386842, 0.003474982, -6.3547e-06,
                      6.96858e-09, -2.50659e-12, -30208.11,
                      2.590233]),
                NASA([1000.0, 5000.0],
                     [2.672146, 0.003056293, -8.73026e-07,
                      1.201e-10, -6.39162e-15, -29899.21,
                      6.862817])),
        transport = gas_transport(
                geom = "nonlinear",
                well_depth = 572.4,
                diam = 2.605,
                dipole = 1.844,
                rot_relax = 4.0))

species(name='HO2',
        atoms='H:1 O:2',
        thermo=(NASA([200.0, 1000.0],
                     [4.30179801, -0.004749121, 2.11583e-05,
                      -2.42764e-08, 9.29225e-12, 294.80804,
                      3.71666245]),
                NASA([1000.0, 3500.0],
                     [4.0172109, 0.00223982, -6.33658e-07,
                      1.14246e-10, -1.07909e-14, 111.856713,
                      3.78510215])),
        transport = gas_transport(
                geom = "nonlinear",
                well_depth = 107.4,
                diam = 3.458,
                rot_relax = 1.0))

species(name='H2O2',
        atoms='H:2 O:2',
        thermo=(NASA([300.0, 1000.0],
                     [3.388754, 0.006569226, -1.48501e-07,
                      -4.62581e-09, 2.47152e-12, -17663.15,
                      6.785363]),
```

```
                NASA([1000.0, 5000.0],
                     [4.573167, 0.004336136, -1.47469e-06,
                      2.3489e-10, -1.43165e-14, -18006.96,
                      0.501137])),
        transport = gas_transport(
                geom = "nonlinear",
                well_depth = 107.4,
                diam = 3.458,
                rot_relax = 3.8))


#--------------------------------------------------------------------------------

#Reaction data
#--------------------------------------------------------------------------------


#Reaction 1:
reaction('O2 + H <=> OH + O', [1.04e+14, 0.0, 15309.835])

#Reaction 2:
reaction('H2 + O <=> OH + H', [8.7923244e+14, 0.0, 19174.55],
         options='duplicate')

#Reaction 3:
reaction('H2 + O <=> OH + H', [3.81803676e+12, 0.0, 7948.0],
         options='duplicate')

#Reaction 4:
reaction('H2 + OH <=> H2O + H', [216194826.0, 1.51, 3429.562])

#Reaction 5:
reaction('OH + OH <=> H2O + O', [2.83e+13, -0.764, -460.560180575],
         options='duplicate')

#Reaction 6:
reaction('OH + OH <=> H2O + O', [12600.0, 2.5308, -1622.91682141],
         options='duplicate')

#Reaction 7:
```

```
three_body_reaction('H + H + M <=> H2 + M', [3.143e+20, -1.806,
   982.555066967],
        efficiencies='H2:2.5 H2O:12.0 CO:1.9 CO2:3.8 Ar:0.0 He:0.0
           ')

#Reaction 8:
reaction('H + H + Ar <=> H2 + Ar', [4.011e+19, -1.506,
   982.555066967])

#Reaction 9:
reaction('H + H + He <=> H2 + He', [4.011e+19, -1.506,
   982.555066967])

#Reaction 10:
three_body_reaction('O + O + M <=> O2 + M', [6.16524893053e+15,
   -0.5, 0.0],
        efficiencies='H2:2.53 H2O:11.76 CO:1.88 CO2:3.82 Ar:0.0 He
           :0.0 ')

#Reaction 11:
reaction('O + O + Ar <=> O2 + Ar', [1.88584084934e+13, 0.0,
   -1788.3])

#Reaction 12:
reaction('O + O + He <=> O2 + He', [1.88584084934e+13, 0.0,
   -1788.3])

#Reaction 13:
three_body_reaction('H + O + M <=> OH + M', [4.71460212335e+18,
   -1.0, 0.0],
        efficiencies='H2:2.54 H2O:12.31 CO:1.92 CO2:3.77 He:0.75 Ar
           :0.75 ')

#Reaction 14:
three_body_reaction('OH + H + M <=> H2O + M', [1.483e+28, -3.798,
   2706.52897774],
        efficiencies='H2:3.0 O2:1.5 N2:2.0 He:1.1 CO:1.9 CO2:3.8
           H2O:0.0 ')

#Reaction 15:
```

```
reaction('OH + H + H2O <=> H2O + H2O', [2.46e+26, -2.916,
    2096.18418054])

#Reaction 16:
falloff_reaction('O2 + H (+ M) <=> HO2 (+ M)',
                 kf=[4.65e+12, 0.44, 0.0],
                 kf0=[6.37e+20, -1.72, 524.568],
                 efficiencies='H2:1.99 O2:0.78 H2O:14.0 CO:1.9 CO2
                     :3.8 Ar:0.67 He:0.8 ',
         falloff = Troe(A = 0.5, T3 = 1e-30, T1 = 1e+30, T2 = 0))

#Reaction 17:
reaction('O2 + H2 <=> HO2 + H', [1341000.0, 2.314, 53420.1782336])

#Reaction 18:
reaction('HO2 + H <=> OH + OH', [7.08e+13, 0.0, 300.169572393])

#Reaction 19:
reaction('HO2 + O <=> OH + O2', [28500000000.0, 1.0,
    -724.309178184])

#Reaction 20:
reaction('O2 + H2O <=> HO2 + OH', [2.642e+20, -2.194,
    70150.6296335],
         options='duplicate')

#Reaction 21:
reaction('O2 + H2O <=> HO2 + OH', [1656000000.0, 1.533,
    68259.5613274],
         options='duplicate')

#Reaction 22:
reaction('HO2 + HO2 <=> H2O2 + O2', [1510.0, 2.6969, -3866.702],
         options='duplicate')

#Reaction 23:
reaction('HO2 + HO2 <=> H2O2 + O2', [2.5e+15, -1.461, -1469.7839],
         options='duplicate')

#Reaction 24:
```

```
falloff_reaction('OH + OH (+ M) <=> H2O2 (+ M)',
               kf=[5.03e+12, 0.058, -634.68854952],
               kf0=[5.68e+25, -3.358, 576.325578995],
               efficiencies='CO2:2.99 N2:2.01 He:0.4 H2O:10.0 ',
        falloff = Troe(A = 0.55, T3 = 1e-30, T1 = 1e+30, T2 = 0))

#Reaction 25:
reaction('H2O2 + H <=> OH + H2O', [2.408856e+13, 0.0, 3974.0])

#Reaction 26:
reaction('H2O2 + H <=> H2 + HO2', [4.817712e+13, 0.0, 7948.0])

#Reaction 27:
reaction('O + H2O2 <=> HO2 + OH', [9635424.0, 2.0, 3974.0])

#Reaction 28:
reaction('OH + H2O2 <=> HO2 + H2O', [1.51e+14, -1.0553,
   -760.929866016],
        options='duplicate')

#Reaction 29:
reaction('OH + H2O2 <=> HO2 + H2O', [2100.0, 2.9565,
   -1358.7675977],
        options='duplicate')
```

*5.3. Mechanism3 - m00000009.cti*

```
#-------------------------------------------------------------------------------

#HDF5
# CTI Generated : 2017-12-02 01:01:14
#-------------------------------------------------------------------------------


units(length='cm', time='s', quantity='mol', act_energy='cal/mol')


ideal_gas(name='gas',
         elements="Ar C H He N O",
         species="""Ar He N2 C(GR) CO
                    CO2 H H2 O O2
                    OH H2O HO2 H2O2 O2(^1Delta)
                    O(1D) O3 OH*""",
         reactions='all',
         initial_state=state(temperature= 298.15, pressure=
            100000.0))

#-------------------------------------------------------------------------------

#Species data
#-------------------------------------------------------------------------------


species(name='Ar',
       atoms='Ar:1',
       thermo=(NASA([300.0, 1000.0],
                   [2.5, 0.0, 0.0,
                    0.0, 0.0, -745.375,
                    4.366001]),
              NASA([1000.0, 5000.0],
                   [2.5, 0.0, 0.0,
                    0.0, 0.0, -745.375,
                    4.366001])),
       transport = gas_transport(
              geom = "atom",
              well_depth = 136.5,
```

```
              diam = 3.33))

species(name='He',
       atoms='He:1',
       thermo=(NASA([300.0, 1000.0],
                   [2.5, 0.0, 0.0,
                    0.0, 0.0, -745.375,
                    0.9153488]),
              NASA([1000.0, 5000.0],
                   [2.5, 0.0, 0.0,
                    0.0, 0.0, -745.375,
                    0.9153488])),
       transport = gas_transport(
              geom = "atom",
              well_depth = 10.2,
              diam = 2.576))

species(name='N2',
       atoms='N:2',
       thermo=(NASA([300.0, 1000.0],
                   [3.298677, 0.00140824, -3.96322e-06,
                    5.64152e-09, -2.44486e-12, -1020.9,
                    3.950372]),
              NASA([1000.0, 5000.0],
                   [2.92664, 0.001487977, -5.68476e-07,
                    1.0097e-10, -6.75335e-15, -922.7977,
                    5.980528])),
       transport = gas_transport(
              geom = "linear",
              well_depth = 97.53,
              diam = 3.621,
              polar = 1.76,
              rot_relax = 4.0))

species(name='C(GR)',
       atoms='C:1',
       thermo=(NASA([200.0, 1000.0],
                   [-0.31087, 0.0044035, 1.9039e-06,
                    -6.3855e-09, 2.9896e-12, -108.6508,
                    1.1138]),
```

```
                NASA([1000.0, 5000.0],
                     [1.4557, 0.0017171, -6.9758e-07,
                      1.3528e-10, -9.6765e-15, -695.128,
                      -8.5257])),
        transport = gas_transport(
                geom = "atom",
                well_depth = 71.4,
                diam = 3.298))

species(name='CO',
        atoms='C:1 O:1',
        thermo=(NASA([300.0, 1000.0],
                     [3.262452, 0.001511941, -3.88176e-06,
                      5.58194e-09, -2.47495e-12, -14310.54,
                      4.848897]),
                NASA([1000.0, 5000.0],
                     [3.025078, 0.001442689, -5.63083e-07,
                      1.01858e-10, -6.91095e-15, -14268.35,
                      6.108218])),
        transport = gas_transport(
                geom = "linear",
                well_depth = 98.1,
                diam = 3.65,
                polar = 1.95,
                rot_relax = 1.8))

species(name='CO2',
        atoms='C:1 O:2',
        thermo=(NASA([300.0, 1000.0],
                     [2.275725, 0.009922072, -1.04091e-05,
                      6.86669e-09, -2.11728e-12, -48373.14,
                      10.18849]),
                NASA([1000.0, 5000.0],
                     [4.453623, 0.003140169, -1.27841e-06,
                      2.394e-10, -1.66903e-14, -48966.96,
                      -0.9553959])),
        transport = gas_transport(
                geom = "linear",
                well_depth = 244.0,
                diam = 3.763,
```

```
                polar = 2.65,
                rot_relax = 2.1))

species(name='H',
        atoms='H:1',
        thermo=(NASA([300.0, 1000.0],
                     [2.5, 0.0, 0.0,
                      0.0, 0.0, 25471.63,
                      -0.4601176]),
                NASA([1000.0, 5000.0],
                     [2.5, 0.0, 0.0,
                      0.0, 0.0, 25471.63,
                      -0.4601176])),
        transport = gas_transport(
                geom = "atom",
                well_depth = 145.0,
                diam = 2.05))

species(name='H2',
        atoms='H:2',
        thermo=(NASA([300.0, 1000.0],
                     [3.298124, 0.000824944, -8.14302e-07,
                      -9.47543e-11, 4.13487e-13, -1012.521,
                      -3.294094]),
                NASA([1000.0, 5000.0],
                     [2.991423, 0.000700064, -5.63383e-08,
                      -9.23158e-12, 1.58275e-15, -835.034,
                      -1.35511])),
        transport = gas_transport(
                geom = "linear",
                well_depth = 38.0,
                diam = 2.92,
                polar = 0.79,
                rot_relax = 280.0))

species(name='O',
        atoms='O:1',
        thermo=(NASA([300.0, 1000.0],
                     [2.946429, -0.001638166, 2.42103e-06,
                      -1.60284e-09, 3.8907e-13, 29147.64,
```

```
                 2.963995]),
             NASA([1000.0, 5000.0],
                 [2.54206, -2.75506e-05, -3.1028e-09,
                  4.55107e-12, -4.36805e-16, 29230.8,
                  4.920308])),
        transport = gas_transport(
             geom = "atom",
             well_depth = 80.0,
             diam = 2.75))

species(name='O2',
        atoms='O:2',
        thermo=(NASA([300.0, 1000.0],
                 [3.212936, 0.001127486, -5.75615e-07,
                  1.31388e-09, -8.76855e-13, -1005.249,
                  6.034738]),
             NASA([1000.0, 5000.0],
                 [3.697578, 0.00061352, -1.25884e-07,
                  1.77528e-11, -1.13644e-15, -1233.93,
                  3.189166])),
        transport = gas_transport(
             geom = "linear",
             well_depth = 107.4,
             diam = 3.458,
             polar = 1.6,
             rot_relax = 3.8))

species(name='OH',
        atoms='H:1 O:1',
        thermo=(NASA([200.0, 1000.0],
                 [4.12530561, -0.003225449, 6.52765e-06,
                  -5.79854e-09, 2.06237e-12, 3346.30913,
                  -0.69043296]),
             NASA([1000.0, 6000.0],
                 [2.86472886, 0.001056504, -2.59083e-07,
                  3.05219e-11, -1.33196e-15, 3683.62875,
                  5.70164073])),
        transport = gas_transport(
             geom = "linear",
             well_depth = 80.0,
```

```
                diam = 2.75))

species(name='H2O',
        atoms='H:2 O:1',
        thermo=(NASA([300.0, 1000.0],
                     [3.386842, 0.003474982, -6.3547e-06,
                      6.96858e-09, -2.50659e-12, -30208.11,
                      2.590233]),
                NASA([1000.0, 5000.0],
                     [2.672146, 0.003056293, -8.73026e-07,
                      1.201e-10, -6.39162e-15, -29899.21,
                      6.862817])),
        transport = gas_transport(
                geom = "nonlinear",
                well_depth = 572.4,
                diam = 2.605,
                dipole = 1.844,
                rot_relax = 4.0))

species(name='HO2',
        atoms='H:1 O:2',
        thermo=(NASA([200.0, 1000.0],
                     [4.30179801, -0.004749121, 2.11583e-05,
                      -2.42764e-08, 9.29225e-12, 294.80804,
                      3.71666245]),
                NASA([1000.0, 3500.0],
                     [4.0172109, 0.00223982, -6.33658e-07,
                      1.14246e-10, -1.07909e-14, 111.856713,
                      3.78510215])),
        transport = gas_transport(
                geom = "nonlinear",
                well_depth = 107.4,
                diam = 3.458,
                rot_relax = 1.0))

species(name='H2O2',
        atoms='H:2 O:2',
        thermo=(NASA([300.0, 1000.0],
                     [3.388754, 0.006569226, -1.48501e-07,
                      -4.62581e-09, 2.47152e-12, -17663.15,
```

```
                6.785363]),
            NASA([1000.0, 5000.0],
                [4.573167, 0.004336136, -1.47469e-06,
                 2.3489e-10, -1.43165e-14, -18006.96,
                 0.501137])),
    transport = gas_transport(
            geom = "nonlinear",
            well_depth = 107.4,
            diam = 3.458,
            rot_relax = 3.8))

species(name='O2(^1Delta)',
    atoms='O:2',
    thermo=(NASA([200.0, 1000.0],
                [3.78535371, -0.0032192854, 1.12323443e-05,
                 -1.17254068e-08, 4.17659585e-12, 10292.2572,
                 3.27320239]),
            NASA([1000.0, 6000.0],
                [3.45852381, 0.00104045351, -2.79664041e-07,
                 3.11439672e-11, -8.55656058e-16, 10222.9063,
                 4.15264119])),
    transport = gas_transport(
            geom = "linear",
            well_depth = 107.4,
            diam = 3.458,
            polar = 1.6,
            rot_relax = 3.8))

species(name='O(1D)',
    atoms='O:1',
    thermo=(NASA([200.0, 1000.0],
                [2.49993786, 1.71935346e-07, -3.45215267e-10,
                 3.71342028e-13, -1.70964494e-16, 51996.5317,
                 4.61684555]),
            NASA([1000.0, 6000.0],
                [2.49368475, 1.37617903e-05, -1.00401058e-08,
                 2.76012182e-12, -2.01597513e-16, 51998.6304,
                 4.6505095])),
    transport = gas_transport(
            geom = "atom",
```

```
                well_depth = 80.0,
                diam = 2.75))

species(name='O3',
        atoms='O:3',
        thermo=(NASA([200.0, 1000.0],
                     [3.4074, 0.0020538, 1.3849e-05,
                      -2.2331e-08, 9.7607e-12, 15864.4979,
                      8.2825]),
                NASA([1000.0, 6000.0],
                     [12.3303, -0.011932, 7.9874e-06,
                      -1.7719e-09, 1.2608e-13, 12675.5831,
                      -40.8823])),
        transport = gas_transport(
                geom = "nonlinear",
                well_depth = 180.0,
                diam = 4.1,
                rot_relax = 2.0))

species(name='OH*',
        atoms='H:1 O:1',
        thermo=(NASA([300.0, 1000.0],
                     [3.46084428, 0.000501872172, -2.00254474e-06,
                      3.18901984e-09, -1.35451838e-12, 50734.9466,
                      1.73976415]),
                NASA([1000.0, 6000.0],
                     [2.7558292, 0.00139848756, -4.19428493e-07,
                      6.33453282e-11, -3.56042218e-15, 50975.1756,
                      5.62581429])),
        transport = gas_transport(
                geom = "linear",
                well_depth = 80.0,
                diam = 2.75))


#-------------------------------------------------------------------------------

#Reaction data
#-------------------------------------------------------------------------------
```

```
#Reaction 1:
reaction('O2 + H <=> OH + O', [1.04e+14, 0.0, 15309.835])

#Reaction 2:
reaction('H2 + O <=> OH + H', [8.7923244e+14, 0.0, 19174.55],
        options='duplicate')

#Reaction 3:
reaction('H2 + O <=> OH + H', [3.81803676e+12, 0.0, 7948.0],
        options='duplicate')

#Reaction 4:
reaction('H2 + OH <=> H2O + H', [216194826.0, 1.51, 3429.562])

#Reaction 5:
reaction('OH + OH <=> H2O + O', [2.83e+13, -0.764, -460.560180575],
        options='duplicate')

#Reaction 6:
reaction('OH + OH <=> H2O + O', [12600.0, 2.5308, -1622.91682141],
        options='duplicate')

#Reaction 7:
three_body_reaction('H + H + M <=> H2 + M', [3.143e+20, -1.806,
   982.555066967],
        efficiencies='H2:2.5 H2O:12.0 CO:1.9 CO2:3.8 Ar:0.0 He:0.0
            ')

#Reaction 8:
reaction('H + H + Ar <=> H2 + Ar', [4.011e+19, -1.506,
   982.555066967])

#Reaction 9:
reaction('H + H + He <=> H2 + He', [4.011e+19, -1.506,
   982.555066967])

#Reaction 10:
three_body_reaction('O + O + M <=> O2 + M', [6.16524893053e+15,
   -0.5, 0.0],
```

```
        efficiencies='H2:2.53 H2O:11.76 CO:1.88 CO2:3.82 Ar:0.0 He
           :0.0 ')

#Reaction 11:
reaction('O + O + Ar <=> O2 + Ar', [1.88584084934e+13, 0.0,
   -1788.3])

#Reaction 12:
reaction('O + O + He <=> O2 + He', [1.88584084934e+13, 0.0,
   -1788.3])

#Reaction 13:
three_body_reaction('H + O + M <=> OH + M', [4.71460212335e+18,
   -1.0, 0.0],
        efficiencies='H2:2.54 H2O:12.31 CO:1.92 CO2:3.77 He:0.75 Ar
           :0.75 ')

#Reaction 14:
three_body_reaction('OH + H + M <=> H2O + M', [1.483e+28, -3.798,
   2706.52897774],
        efficiencies='H2:3.0 O2:1.5 N2:2.0 He:1.1 CO:1.9 CO2:3.8
           H2O:0.0 ')

#Reaction 15:
reaction('OH + H + H2O <=> H2O + H2O', [2.46e+26, -2.916,
   2096.18418054])

#Reaction 16:
falloff_reaction('O2 + H (+ M) <=> HO2 (+ M)',
               kf=[4.65e+12, 0.44, 0.0],
               kf0=[6.37e+20, -1.72, 524.568],
               efficiencies='H2:1.99 O2:0.78 H2O:14.0 CO:1.9 CO2
                  :3.8 Ar:0.67 He:0.8 ',
        falloff = Troe(A = 0.5, T3 = 1e-30, T1 = 1e+30, T2 = 0))

#Reaction 17:
reaction('O2 + H2 <=> HO2 + H', [1341000.0, 2.314, 53420.1782336])

#Reaction 18:
reaction('HO2 + H <=> OH + OH', [7.08e+13, 0.0, 300.169572393])
```

```
#Reaction 19:
reaction('HO2 + O <=> OH + O2', [28500000000.0, 1.0,
    -724.309178184])

#Reaction 20:
reaction('O2 + H2O <=> HO2 + OH', [2.642e+20, -2.194,
    70150.6296335],
         options='duplicate')

#Reaction 21:
reaction('O2 + H2O <=> HO2 + OH', [1656000000.0, 1.533,
    68259.5613274],
         options='duplicate')

#Reaction 22:
reaction('HO2 + HO2 <=> H2O2 + O2', [1510.0, 2.6969, -3866.702],
         options='duplicate')

#Reaction 23:
reaction('HO2 + HO2 <=> H2O2 + O2', [2.5e+15, -1.461, -1469.7839],
         options='duplicate')

#Reaction 24:
falloff_reaction('OH + OH (+ M) <=> H2O2 (+ M)',
                kf=[5.03e+12, 0.058, -634.68854952],
                kf0=[5.68e+25, -3.358, 576.325578995],
                efficiencies='CO2:2.99 N2:2.01 He:0.4 H2O:10.0 ',
         falloff = Troe(A = 0.55, T3 = 1e-30, T1 = 1e+30, T2 = 0))

#Reaction 25:
reaction('H2O2 + H <=> OH + H2O', [2.408856e+13, 0.0, 3974.0])

#Reaction 26:
reaction('H2O2 + H <=> H2 + HO2', [4.817712e+13, 0.0, 7948.0])

#Reaction 27:
reaction('O + H2O2 <=> HO2 + OH', [9635424.0, 2.0, 3974.0])

#Reaction 28:
```

```
reaction('OH + H2O2 <=> HO2 + H2O', [1.51e+14, -1.0553,
    -760.929866016],
         options='duplicate')

#Reaction 29:
reaction('OH + H2O2 <=> HO2 + H2O', [2100.0, 2.9565,
    -1358.7675977],
         options='duplicate')

#Reaction 30:
three_body_reaction('O3 + M <=> O2 + O + M', [4054000.0, 0.0,
    24416.256],
         efficiencies='Ar:0.51 O2:0.95 O3:2.5 O:4.0 ')

#Reaction 31:
reaction('O3 + O <=> O2 + O2', [4.817712e+12, 0.0, 4093.22])

#Reaction 32:
reaction('O3 + O <=> O2(^1Delta) + O2', [144531360000.0, 0.0,
    4093.22])

#Reaction 33:
three_body_reaction('O + O + M <=> O2(^1Delta) + M', [7e+15, -1.0,
    0.0],
         efficiencies='O:28.86 O2:8.0 H2O:5.0 O3:8.0 N2:2.0 ')

#Reaction 34:
three_body_reaction('O2(^1Delta) + M <=> O2 + M', [1806642.0, 0.0,
    397.4],
         efficiencies='Ar:0.01 He:0.01 CO2:0.01 H2O:3.3 H2:2.5 CO
             :5.67 O:43.33 H:21833333.33 N2:0.0 ')

#Reaction 35:
three_body_reaction('O2(^1Delta) + O + M <=> O2 + O + M',
    [3.62661701796e+15, 0.0, 0.0],
         efficiencies='Ar:0.63 ')

#Reaction 36:
reaction('O2(^1Delta) + O3 <=> O2 + O2 + O', [3.1315128e+13, 0.0,
    5643.08])
```

```
#Reaction 37:
reaction('O2(^1Delta) + O(1D) <=> O2 + O', [6.03e+12, 0.0, 0.0])

#Reaction 38:
reaction('O2 + O(1D) <=> O2(^1Delta) + O', [1.9270848e+13, 0.0,
   -133.129])

#Reaction 39:
three_body_reaction('O(1D) + M <=> O + M', [481771200000.0, 0.0,
   0.0],
        efficiencies='O2:5.83 O:10.0 H2O:3.0 N2:26.15 ')

#Reaction 40:
reaction('O(1D) + O3 <=> O2 + O + O', [7.226568e+13, 0.0, 0.0])

#Reaction 41:
reaction('O(1D) + O3 <=> O2 + O2', [7.226568e+13, 0.0, 0.0])

#Reaction 42:
reaction('H2 + O2(^1Delta) <=> H + HO2', [616000.0, 2.335,
   31097.5676999])

#Reaction 43:
reaction('O2(^1Delta) + H <=> OH + O', [349886334.0, 1.45,
   4510.49])

#Reaction 44:
three_body_reaction('H + O2(^1Delta) + M <=> HO2 + M',
   [9890000000.0, 2.03, 3360.017],
        efficiencies='')

#Reaction 45:
reaction('HO2 + OH <=> H2O + O2(^1Delta)', [109300.0, 1.707,
   12542.0852998])

#Reaction 46:
reaction('OH + O2(^1Delta) <=> O + HO2', [1.3e+13, 0.0,
   34019.2182045])
```

```
#Reaction 47:
reaction('O3 + H <=> OH + O2', [8.430996e+13, 0.0, 933.89])

#Reaction 48:
reaction('OH + O3 <=> HO2 + O2', [1.7e-12, 0.0, 1867.78])

#Reaction 49:
reaction('HO2 + O3 <=> OH + O2 + O2', [0.000584749794, 4.57,
   -1376.991])

#Reaction 50:
reaction('H + HO2 <=> H2O + O(1D)', [2.5e+12, 0.0, 300.169572393])

#Reaction 51:
reaction('O(1D) + H2 <=> OH + H', [8.129889e+13, 0.0, 0.0])

#Reaction 52:
reaction('O(1D) + H2O <=> OH + OH', [1.0237638e+14, 0.0, -71.532])

#Reaction 53:
three_body_reaction('O + H + M <=> OH* + M', [1.5e+13, 0.0,
   5974.52960908],
        efficiencies='O2:0.4 Ar:0.35 N2:0.4 H2O:6.5 ')

#Reaction 54:
three_body_reaction('OH* + M <=> OH + M', [21470000000.0, 0.5,
   2061.1643971],
        efficiencies='O2:39.12 N2:5.03 H2O:137.87 H2:16.49 OH:69.86
            H:69.86 O:69.86 ')

#Reaction 55:
reaction('OH* + H2 <=> H2O + H', [2.6e+12, 0.5, -444.250967142])

#Reaction 56:
reaction('OH* + O2 <=> O3 + H', [252000000000.0, 0.5,
   -482.272446312])

#Reaction 57:
reaction('OH* + O2 <=> HO2 + O', [1.008e+12, 0.5, -482.272446312])
```

```
#Reaction 58:
reaction('OH* + H2O <=> H2O2 + H', [2.96e+12, 0.5, -861.486672768])
```

*5.4. DynamicMech151203 - m00000010.cti*

```
#--------------------------------------------------------------------------------

#HDF5
# CTI Generated : 2017-12-02 01:06:32
#--------------------------------------------------------------------------------


units(length='cm', time='s', quantity='mol', act_energy='cal/mol')


ideal_gas(name='gas',
          elements="Ar C H He N O",
          species="""Ar He N2 C(GR) CO
                     CO2 H H2 O O2
                     OH H2O HO2 H2O2 O2(^1Delta)
                     O(1D) O3 OH*""",
          reactions='all',
          initial_state=state(temperature= 298.15, pressure=
              100000.0))

#--------------------------------------------------------------------------------

#Species data
#--------------------------------------------------------------------------------


species(name='Ar',
        atoms='Ar:1',
        thermo=(NASA([300.0, 1000.0],
                     [2.5, 0.0, 0.0,
                      0.0, 0.0, -745.375,
                      4.366001]),
                NASA([1000.0, 5000.0],
                     [2.5, 0.0, 0.0,
                      0.0, 0.0, -745.375,
                      4.366001])),
        transport = gas_transport(
                geom = "atom",
                well_depth = 136.5,
```

```
              diam = 3.33))

species(name='He',
        atoms='He:1',
        thermo=(NASA([300.0, 1000.0],
                     [2.5, 0.0, 0.0,
                      0.0, 0.0, -745.375,
                      0.9153488]),
                NASA([1000.0, 5000.0],
                     [2.5, 0.0, 0.0,
                      0.0, 0.0, -745.375,
                      0.9153488])),
        transport = gas_transport(
                geom = "atom",
                well_depth = 10.2,
                diam = 2.576))

species(name='N2',
        atoms='N:2',
        thermo=(NASA([300.0, 1000.0],
                     [3.298677, 0.00140824, -3.96322e-06,
                      5.64152e-09, -2.44486e-12, -1020.9,
                      3.950372]),
                NASA([1000.0, 5000.0],
                     [2.92664, 0.001487977, -5.68476e-07,
                      1.0097e-10, -6.75335e-15, -922.7977,
                      5.980528])),
        transport = gas_transport(
                geom = "linear",
                well_depth = 97.53,
                diam = 3.621,
                polar = 1.76,
                rot_relax = 4.0))

species(name='C(GR)',
        atoms='C:1',
        thermo=(NASA([200.0, 1000.0],
                     [-0.31087, 0.0044035, 1.9039e-06,
                      -6.3855e-09, 2.9896e-12, -108.6508,
                      1.1138]),
```

```
            NASA([1000.0, 5000.0],
                 [1.4557, 0.0017171, -6.9758e-07,
                  1.3528e-10, -9.6765e-15, -695.128,
                  -8.5257])),
        transport = gas_transport(
            geom = "atom",
            well_depth = 71.4,
            diam = 3.298))

species(name='CO',
        atoms='C:1 O:1',
        thermo=(NASA([300.0, 1000.0],
                 [3.262452, 0.001511941, -3.88176e-06,
                  5.58194e-09, -2.47495e-12, -14310.54,
                  4.848897]),
            NASA([1000.0, 5000.0],
                 [3.025078, 0.001442689, -5.63083e-07,
                  1.01858e-10, -6.91095e-15, -14268.35,
                  6.108218])),
        transport = gas_transport(
            geom = "linear",
            well_depth = 98.1,
            diam = 3.65,
            polar = 1.95,
            rot_relax = 1.8))

species(name='CO2',
        atoms='C:1 O:2',
        thermo=(NASA([300.0, 1000.0],
                 [2.275725, 0.009922072, -1.04091e-05,
                  6.86669e-09, -2.11728e-12, -48373.14,
                  10.18849]),
            NASA([1000.0, 5000.0],
                 [4.453623, 0.003140169, -1.27841e-06,
                  2.394e-10, -1.66903e-14, -48966.96,
                  -0.9553959])),
        transport = gas_transport(
            geom = "linear",
            well_depth = 244.0,
            diam = 3.763,
```

```
                polar = 2.65,
                rot_relax = 2.1))

species(name='H',
        atoms='H:1',
        thermo=(NASA([300.0, 1000.0],
                     [2.5, 0.0, 0.0,
                      0.0, 0.0, 25471.63,
                      -0.4601176]),
                NASA([1000.0, 5000.0],
                     [2.5, 0.0, 0.0,
                      0.0, 0.0, 25471.63,
                      -0.4601176])),
        transport = gas_transport(
                geom = "atom",
                well_depth = 145.0,
                diam = 2.05))

species(name='H2',
        atoms='H:2',
        thermo=(NASA([300.0, 1000.0],
                     [3.298124, 0.000824944, -8.14302e-07,
                      -9.47543e-11, 4.13487e-13, -1012.521,
                      -3.294094]),
                NASA([1000.0, 5000.0],
                     [2.991423, 0.000700064, -5.63383e-08,
                      -9.23158e-12, 1.58275e-15, -835.034,
                      -1.35511])),
        transport = gas_transport(
                geom = "linear",
                well_depth = 38.0,
                diam = 2.92,
                polar = 0.79,
                rot_relax = 280.0))

species(name='O',
        atoms='O:1',
        thermo=(NASA([300.0, 1000.0],
                     [2.946429, -0.001638166, 2.42103e-06,
                      -1.60284e-09, 3.8907e-13, 29147.64,
```

```
                   2.963995]),
            NASA([1000.0, 5000.0],
                  [2.54206, -2.75506e-05, -3.1028e-09,
                   4.55107e-12, -4.36805e-16, 29230.8,
                   4.920308])),
        transport = gas_transport(
            geom = "atom",
            well_depth = 80.0,
            diam = 2.75))

species(name='O2',
        atoms='O:2',
        thermo=(NASA([300.0, 1000.0],
                  [3.212936, 0.001127486, -5.75615e-07,
                   1.31388e-09, -8.76855e-13, -1005.249,
                   6.034738]),
            NASA([1000.0, 5000.0],
                  [3.697578, 0.00061352, -1.25884e-07,
                   1.77528e-11, -1.13644e-15, -1233.93,
                   3.189166])),
        transport = gas_transport(
            geom = "linear",
            well_depth = 107.4,
            diam = 3.458,
            polar = 1.6,
            rot_relax = 3.8))

species(name='OH',
        atoms='H:1 O:1',
        thermo=(NASA([200.0, 1000.0],
                  [4.12530561, -0.003225449, 6.52765e-06,
                   -5.79854e-09, 2.06237e-12, 3346.30913,
                   -0.69043296]),
            NASA([1000.0, 6000.0],
                  [2.86472886, 0.001056504, -2.59083e-07,
                   3.05219e-11, -1.33196e-15, 3683.62875,
                   5.70164073])),
        transport = gas_transport(
            geom = "linear",
            well_depth = 80.0,
```

```
                diam = 2.75))

species(name='H2O',
        atoms='H:2 O:1',
        thermo=(NASA([300.0, 1000.0],
                     [3.386842, 0.003474982, -6.3547e-06,
                      6.96858e-09, -2.50659e-12, -30208.11,
                      2.590233]),
                NASA([1000.0, 5000.0],
                     [2.672146, 0.003056293, -8.73026e-07,
                      1.201e-10, -6.39162e-15, -29899.21,
                      6.862817])),
        transport = gas_transport(
                geom = "nonlinear",
                well_depth = 572.4,
                diam = 2.605,
                dipole = 1.844,
                rot_relax = 4.0))

species(name='HO2',
        atoms='H:1 O:2',
        thermo=(NASA([200.0, 1000.0],
                     [4.30179801, -0.004749121, 2.11583e-05,
                      -2.42764e-08, 9.29225e-12, 294.80804,
                      3.71666245]),
                NASA([1000.0, 3500.0],
                     [4.0172109, 0.00223982, -6.33658e-07,
                      1.14246e-10, -1.07909e-14, 111.856713,
                      3.78510215])),
        transport = gas_transport(
                geom = "nonlinear",
                well_depth = 107.4,
                diam = 3.458,
                rot_relax = 1.0))

species(name='H2O2',
        atoms='H:2 O:2',
        thermo=(NASA([300.0, 1000.0],
                     [3.388754, 0.006569226, -1.48501e-07,
                      -4.62581e-09, 2.47152e-12, -17663.15,
```

```
                 6.785363]),
             NASA([1000.0, 5000.0],
                 [4.573167, 0.004336136, -1.47469e-06,
                  2.3489e-10, -1.43165e-14, -18006.96,
                  0.501137])),
        transport = gas_transport(
                geom = "nonlinear",
                well_depth = 107.4,
                diam = 3.458,
                rot_relax = 3.8))

species(name='O2(^1Delta)',
        atoms='O:2',
        thermo=(NASA([200.0, 1000.0],
                 [3.78535371, -0.0032192854, 1.12323443e-05,
                  -1.17254068e-08, 4.17659585e-12, 10292.2572,
                  3.27320239]),
             NASA([1000.0, 6000.0],
                 [3.45852381, 0.00104045351, -2.79664041e-07,
                  3.11439672e-11, -8.55656058e-16, 10222.9063,
                  4.15264119])),
        transport = gas_transport(
                geom = "linear",
                well_depth = 107.4,
                diam = 3.458,
                polar = 1.6,
                rot_relax = 3.8))

species(name='O(1D)',
        atoms='O:1',
        thermo=(NASA([200.0, 1000.0],
                 [2.49993786, 1.71935346e-07, -3.45215267e-10,
                  3.71342028e-13, -1.70964494e-16, 51996.5317,
                  4.61684555]),
             NASA([1000.0, 6000.0],
                 [2.49368475, 1.37617903e-05, -1.00401058e-08,
                  2.76012182e-12, -2.01597513e-16, 51998.6304,
                  4.6505095])),
        transport = gas_transport(
                geom = "atom",
```

```
                well_depth = 80.0,
                diam = 2.75))

species(name='O3',
        atoms='O:3',
        thermo=(NASA([200.0, 1000.0],
                     [3.4074, 0.0020538, 1.3849e-05,
                      -2.2331e-08, 9.7607e-12, 15864.4979,
                      8.2825]),
                NASA([1000.0, 6000.0],
                     [12.3303, -0.011932, 7.9874e-06,
                      -1.7719e-09, 1.2608e-13, 12675.5831,
                      -40.8823])),
        transport = gas_transport(
                geom = "nonlinear",
                well_depth = 180.0,
                diam = 4.1,
                rot_relax = 2.0))

species(name='OH*',
        atoms='H:1 O:1',
        thermo=(NASA([300.0, 1000.0],
                     [3.46084428, 0.000501872172, -2.00254474e-06,
                      3.18901984e-09, -1.35451838e-12, 50734.9466,
                      1.73976415]),
                NASA([1000.0, 6000.0],
                     [2.7558292, 0.00139848756, -4.19428493e-07,
                      6.33453282e-11, -3.56042218e-15, 50975.1756,
                      5.62581429])),
        transport = gas_transport(
                geom = "linear",
                well_depth = 80.0,
                diam = 2.75))


#-------------------------------------------------------------------------------

#Reaction data
#-------------------------------------------------------------------------------
```

```
#Reaction 1:
reaction('O2 + H <=> OH + O', [1.0426e+14, 0.0, 15309.835])

#Reaction 2:
reaction('H2 + O <=> OH + H', [1.1163843132e+15, 0.0, 19174.55],
        options='duplicate')

#Reaction 3:
reaction('H2 + O <=> OH + H', [4.8478829214e+12, 0.0, 7948.0],
        options='duplicate')

#Reaction 4:
reaction('H2 + OH <=> H2O + H', [189661277.16, 1.51, 3429.562])

#Reaction 5:
reaction('OH + OH <=> H2O + O', [2.83e+13, -0.764, -460.560180575],
        options='duplicate')

#Reaction 6:
reaction('OH + OH <=> H2O + O', [12600.0, 2.5308, -1622.91682141],
        options='duplicate')

#Reaction 7:
three_body_reaction('H + H + M <=> H2 + M', [3.143e+20, -1.806,
    982.555066967],
        efficiencies='H2:2.5 H2O:12.0 CO:1.9 CO2:3.8 Ar:0.0 He:0.0
            ')

#Reaction 8:
reaction('H + H + Ar <=> H2 + Ar', [4.011e+19, -1.506,
    982.555066967])

#Reaction 9:
reaction('H + H + He <=> H2 + He', [4.011e+19, -1.506,
    982.555066967])

#Reaction 10:
three_body_reaction('O + O + M <=> O2 + M', [3.56641517546e+15,
    -0.5, 0.0],
```

```
        efficiencies='H2:2.53 H2O:11.76 CO:1.88 CO2:3.82 Ar:0.0 He
            :0.0 ')

#Reaction 11:
reaction('O + O + Ar <=> O2 + Ar', [1.090886399e+13, 0.0, -1788.3])

#Reaction 12:
reaction('O + O + He <=> O2 + He', [1.090886399e+13, 0.0, -1788.3])

#Reaction 13:
three_body_reaction('H + O + M <=> OH + M', [1.56619082538e+18,
    -1.0, 0.0],
        efficiencies='H2:2.54 H2O:12.31 CO:1.92 CO2:3.77 He:0.75 Ar
            :0.75 ')

#Reaction 14:
three_body_reaction('OH + H + M <=> H2O + M', [1.483e+28, -3.798,
    2706.52897774],
        efficiencies='H2:3.0 O2:1.5 N2:2.0 He:1.1 CO:1.9 CO2:3.8
            H2O:0.0 ')

#Reaction 15:
reaction('OH + H + H2O <=> H2O + H2O', [2.46e+26, -2.916,
    2096.18418054])

#Reaction 16:
falloff_reaction('O2 + H (+ M) <=> HO2 (+ M)',
               kf=[3.6934e+12, 0.44, 0.0],
               kf0=[5.0595e+20, -1.72, 524.568],
               efficiencies='H2:1.99 O2:0.78 H2O:14.0 CO:1.9 CO2
                   :3.8 Ar:0.67 He:0.8 ',
        falloff = Troe(A = 0.5, T3 = 1e-30, T1 = 1e+30, T2 = 0))

#Reaction 17:
reaction('O2 + H2 <=> HO2 + H', [823890.0, 2.314, 53420.1782336])

#Reaction 18:
reaction('HO2 + H <=> OH + OH', [1.1333e+14, 0.0, 300.169572393])

#Reaction 19:
```

```
reaction('HO2 + O <=> OH + O2', [24613000000.0, 1.0,
    -724.309178184])

#Reaction 20:
reaction('O2 + H2O <=> HO2 + OH', [2.642e+20, -2.194,
    70150.6296335],
         options='duplicate')

#Reaction 21:
reaction('O2 + H2O <=> HO2 + OH', [1656000000.0, 1.533,
    68259.5613274],
         options='duplicate')

#Reaction 22:
reaction('HO2 + HO2 <=> H2O2 + O2', [1510.0, 2.6969, -3866.702],
         options='duplicate')

#Reaction 23:
reaction('HO2 + HO2 <=> H2O2 + O2', [2.5e+15, -1.461, -1469.7839],
         options='duplicate')

#Reaction 24:
falloff_reaction('OH + OH (+ M) <=> H2O2 (+ M)',
                 kf=[5.03e+12, 0.058, -634.68854952],
                 kf0=[5.68e+25, -3.358, 576.325578995],
                 efficiencies='CO2:2.99 N2:2.01 He:0.4 H2O:10.0 ',
         falloff = Troe(A = 0.55, T3 = 1e-30, T1 = 1e+30, T2 = 0))

#Reaction 25:
reaction('H2O2 + H <=> OH + H2O', [3.9240866454e+13, 0.0, 3974.0])

#Reaction 26:
reaction('H2O2 + H <=> H2 + HO2', [9.801635064e+13, 0.0, 7948.0])

#Reaction 27:
reaction('O + H2O2 <=> HO2 + OH', [5728380.0108, 2.0, 3974.0])

#Reaction 28:
reaction('OH + H2O2 <=> HO2 + H2O', [1.51e+14, -1.0553,
    -760.929866016],
```

```
        options='duplicate')

#Reaction 29:
reaction('OH + H2O2 <=> HO2 + H2O', [2100.0, 2.9565,
    -1358.7675977],
        options='duplicate')

#Reaction 30:
three_body_reaction('O3 + M <=> O2 + O + M', [3332100.0, 0.0,
    24416.256],
        efficiencies='Ar:0.51 O2:0.95 O3:2.5 O:4.0 ')

#Reaction 31:
reaction('O3 + O <=> O2 + O2', [5.5400074716e+12, 0.0, 4093.22])

#Reaction 32:
reaction('O3 + O <=> O2(^1Delta) + O2', [433594080000.0, 0.0,
    4093.22])

#Reaction 33:
three_body_reaction('O + O + M <=> O2(^1Delta) + M', [2.331e+15,
    -1.0, 0.0],
        efficiencies='O:28.86 O2:8.0 H2O:5.0 O3:8.0 N2:2.0 ')

#Reaction 34:
three_body_reaction('O2(^1Delta) + M <=> O2 + M', [1400809.9854,
    0.0, 397.4],
        efficiencies='Ar:0.0 He:0.0 CO2:0.01 H2O:3.3 H2:2.5 CO:5.67
            O:43.33 H:21830531.79 N2:0.0 ')

#Reaction 35:
three_body_reaction('O2(^1Delta) + O + M <=> O2 + O + M',
    [3.62661701796e+15, 0.0, 0.0],
        efficiencies='Ar:0.63 ')

#Reaction 36:
reaction('O2(^1Delta) + O3 <=> O2 + O2 + O', [3.1315128e+13, 0.0,
    5643.08])

#Reaction 37:
```

```
reaction('O2(^1Delta) + O(1D) <=> O2 + O', [6.03e+13, 0.0, 0.0])

#Reaction 38:
reaction('O2 + O(1D) <=> O2(^1Delta) + O', [1.9270848e+13, 0.0,
    -133.129])

#Reaction 39:
three_body_reaction('O(1D) + M <=> O + M', [96354240000.0, 0.0,
    0.0],
         efficiencies='O2:5.83 O:10.0 H2O:3.0 N2:26.15 ')

#Reaction 40:
reaction('O(1D) + O3 <=> O2 + O + O', [7.226568e+13, 0.0, 0.0])

#Reaction 41:
reaction('O(1D) + O3 <=> O2 + O2', [7.226568e+13, 0.0, 0.0])

#Reaction 42:
reaction('H2 + O2(^1Delta) <=> H + HO2', [616000.0, 2.335,
    31097.5676999])

#Reaction 43:
reaction('O2(^1Delta) + H <=> OH + O', [146277780.6, 1.45,
    4510.49])

#Reaction 44:
three_body_reaction('H + O2(^1Delta) + M <=> HO2 + M',
    [95016000000.0, 2.03, 3360.017],
         efficiencies='')

#Reaction 45:
reaction('HO2 + OH <=> H2O + O2(^1Delta)', [327900.0, 1.707,
    12542.0852998])

#Reaction 46:
reaction('OH + O2(^1Delta) <=> O + HO2', [5.8552e+12, 0.0,
    34019.2182045])

#Reaction 47:
reaction('O3 + H <=> OH + O2', [8.430996e+13, 0.0, 933.89])
```

```
#Reaction 48:
reaction('OH + O3 <=> HO2 + O2', [1.7e-12, 0.0, 1867.78])

#Reaction 49:
reaction('HO2 + O3 <=> OH + O2 + O2', [0.00036547163232, 4.57,
   -1376.991])

#Reaction 50:
reaction('H + HO2 <=> H2O + O(1D)', [1.9532e+12, 0.0,
   300.169572393])

#Reaction 51:
reaction('O(1D) + H2 <=> OH + H', [8.129889e+13, 0.0, 0.0])

#Reaction 52:
reaction('O(1D) + H2O <=> OH + OH', [1.0237638e+14, 0.0, -71.532])

#Reaction 53:
three_body_reaction('O + H + M <=> OH* + M', [1.2566e+13, 0.0,
   5974.52960908],
        efficiencies='O2:0.4 Ar:0.35 N2:0.4 H2O:6.5 ')

#Reaction 54:
three_body_reaction('OH* + M <=> OH + M', [21470000000.0, 0.5,
   2061.1643971],
        efficiencies='O2:39.12 N2:5.03 H2O:137.87 H2:16.49 OH:69.86
            H:69.86 O:69.86 ')

#Reaction 55:
reaction('OH* + H2 <=> H2O + H', [2.6e+12, 0.5, -444.250967142])

#Reaction 56:
reaction('OH* + O2 <=> O3 + H', [361410000000.0, 0.5,
   -482.272446312])

#Reaction 57:
reaction('OH* + O2 <=> HO2 + O', [672310000000.0, 0.5,
   -482.272446312])
```

```
#Reaction 58:
reaction('OH* + H2O <=> H2O2 + H', [6.5803e+12, 0.5,
    -861.486672768])
```
